# Supplementary material for: A Mountaineering Strategy to Excited States: Highly-Accurate Reference Energies and Benchmarks
Source: arXiv:1807.02045 source file (2018-07-05)
Supplement: Supplementary file 1 [file FCI-SI.pdf]

# A Mountaineering Strategy to Excited States: Highly-Accurate Reference Energies and Benchmarks

# Supporting Information

Pierre-François Loos,[*,†] Anthony Scemama,[†] Aymeric Blondel,[‡] Yann Garniron,[†] Michel Caffarel,[†] and Denis Jacquemin[*,‡]

†*Laboratoire de Chimie et Physique Quantiques, Université de Toulouse, CNRS, UPS, France*

‡*Laboratoire CEISAM - UMR CNRS 6230, Université de Nantes, 2 Rue de la Houssinière, BP 92208, 44322 Nantes Cedex 3, France*

E-mail: loos@irsamc.ups-tlse.fr; Denis.Jacquemin@univ-nantes.fr

# S1 Basis set and frozen-core effects

## S1.1 Water, ammonia and hydrogen chloride

Table S1: CC3 vertical transition energies of water, hydrogen sulfide, ammonia, and hydrogen chloride using various atomic basis sets. FC stands for frozen core (large frozen core for sulfur and chlorine). All values are in eV.

| | *aug*-cc-pVDZ | *aug*-cc-pVTZ | d-*aug*-cc-pVTZ | *aug*-cc-pVQZ | | d-*aug*-cc-pVQZ | | t-*aug*-cc-pVQZ | | *aug*-cc-pV5Z | d-*aug*-cc-pV5Z |
|---|---|---|---|---|---|---|---|---|---|---|---|
| | FC | FC | FC | FC | Full | FC | Full | FC | Full | Full | Full |
| | Water | | | | | | | | | | |
| $^1B_1(n \rightarrow 3s)$ | 7.51 | 7.60 | 7.60 | 7.65 | 7.66 | 7.65 | 7.66 | 7.64 | 7.66 | 7.67 | 7.67 |
| $^1A_2(n \rightarrow 3p)$ | 9.29 | 9.38 | 9.37 | 9.43 | 9.43 | 9.42 | 9.42 | 9.42 | 9.42 | 9.44 | 9.44 |
| $^1A_1(n \rightarrow 3s)$ | 9.92 | 9.97 | 9.89 | 10.00 | 10.00 | 9.94 | 9.94 | 9.93 | 9.94 | 10.00 | 9.95 |
| $^3B_1(n \rightarrow 3s)$ | 7.13 | 7.23 | 7.23 | 7.28 | 7.29 | 7.28 | 7.29 | 7.28 | 7.29 | 7.31 | 7.31 |
| $^3A_2(n \rightarrow 3p)$ | 9.12 | 9.22 | 9.30 | 9.26 | 9.27 | 9.26 | 9.26 | 9.26 | 9.26 | 9.28 | 9.28 |
| $^3A_1(n \rightarrow 3s)$ | 9.47 | 9.52 | 9.52 | 9.56 | 9.56 | 9.56 | 9.56 | 9.56 | 9.56 | 9.57 | 9.57 |
| | Hydrogen sulfide | | | | | | | | | | |
| $^1A_2(n \rightarrow 4p)$ | 6.29 | 6.19 | 6.17 | 6.16 | 6.15 | 6.15 | 6.14 | 6.15 | 6.14 | 6.12 | 6.11 |
| $^1B_1(n \rightarrow 4s)$ | 6.10 | 6.24 | 6.24 | 6.29 | 6.28 | 6.29 | 6.27 | 6.29 | 6.27 | 6.29 | 6.29 |
| $^3A_2(n \rightarrow 4p)$ | 5.91 | 5.82 | 5.81 | 5.80 | 5.79 | 5.80 | 5.79 | 5.80 | 5.79 | 5.76 | 5.75 |
| $^3B_1(n \rightarrow 4s)$ | 5.75 | 5.88 | 5.88 | 5.93 | 5.92 | 5.93 | 5.92 | 5.93 | 5.92 | 5.94 | 5.94 |
| | Ammonia | | | | | | | | | | |
| $^1A_2(n \rightarrow 3s)$ | 6.46 | 6.57 | 6.57 | 6.61 | 6.61 | 6.61 | 6.61 | 6.61 | 6.61 | 6.63 | 6.63 |
| $^1E(n \rightarrow 3p)$ | 8.06 | 8.15 | 8.12 | 8.18 | 8.18 | 8.16 | 8.16 | 8.16 | 8.16 | 8.18 | 8.17 |
| $^1A_1(n \rightarrow 3p)$ | 9.66 | 9.32 | 8.56 | 9.11 | 9.11 | 8.61 | 8.61 | 8.60 | 8.60 | 8.91 | 8.62 |
| $^1A_2(n \rightarrow 4s)$ | 10.40 | 9.95 | 9.12 | 9.77 | 9.77 | 9.16 | 9.17 | 9.15 | 9.16 | 9.61 | 9.18 |
| $^3A_2(n \rightarrow 3s)$ | 6.18 | 6.29 | 6.29 | 6.33 | 6.34 | 6.33 | 6.34 | 6.33 | 6.34 | 6.35 | 6.35 |
| | Hydrogen chloride | | | | | | | | | | |
| $^1\Pi$(CT) | 7.82 | 7.84 | 7.83 | 7.89 | 7.87 | 7.88 | 7.87 | 7.88 | 7.87 | 7.87 | 7.87 |

## S1.2 Dinitrogen and carbon monoxide

Table S2: CC3 vertical transition energies of dinitrogen (top) and carbon monoxide (bottom) using various atomic basis sets. See caption of Table S1 for more details.

| | *aug*-cc-pVDZ | *aug*-cc-pVTZ | *aug*-cc-pVQZ | | d-*aug*-cc-pVQZ | | t-*aug*-cc-pVQZ | | *aug*-cc-pV5Z | d-*aug*-cc-pV5Z |
|---|---|---|---|---|---|---|---|---|---|---|
| | FC | FC | FC | Full | FC | Full | FC | Full | Full | Full |
| | Dinitrogen | | | | | | | | | |
| $^1\Pi_g(\text{V}; n \to \pi^\star)$ | 9.44 | 9.34 | 9.33 | 9.32 | 9.33 | 9.32 | 9.33 | 9.32 | 9.32 | 9.32 |
| $^1\Sigma_u^-(\text{V}; \pi \to \pi^\star)$ | 10.06 | 9.88 | 9.87 | 9.87 | 9.87 | 9.87 | 9.87 | 9.87 | 9.86 | 9.86 |
| $^1\Delta_u(\text{V}; \pi \to \pi^\star)$ | 10.43 | 10.29 | 10.27 | 10.27 | 10.27 | 10.27 | 10.27 | 10.27 | 10.27 | 10.27 |
| $^1\Sigma_g^+(\text{R}; n \to \sigma^\star)$ | 13.23 | 13.01 | 12.90 | 12.91 | 12.27 | 12.28 | 12.27 | 12.28 | 12.77 | 12.31 |
| $^1\Pi_u(\text{R})$ | 13.28 | 13.22 | 13.17 | 13.16 | 12.89 | 12.90 | 12.89 | 12.90 | 13.08 | 12.92 |
| $^1\Sigma_u^+(\text{R}; n \to \sigma^\star)$ | 13.14 | 13.12 | 13.09 | 13.10 | 12.94 | 12.96 | 12.94 | 12.96 | 13.06 | 12.98 |
| $^1\Pi_u(\text{R})$ | 13.64 | 13.49 | 13.42 | 13.40 | 13.34 | 13.31 | 13.34 | 13.31 | 13.34 | 13.30 |
| $^3\Sigma_u^+(\text{V}; \pi \to \pi^\star)$ | 7.67 | 7.68 | 7.71 | 7.70 | 7.71 | 7.70 | 7.71 | 7.70 | 7.71 | 7.71 |
| $^3\Pi_g(\text{V}; n \to \pi^\star)$ | 8.07 | 8.04 | 8.04 | 8.03 | 8.04 | 8.03 | 8.04 | 8.03 | 8.04 | 8.04 |
| $^3\Delta_u(\text{V}; \pi \to \pi^\star)$ | 8.97 | 8.87 | 8.87 | 8.86 | 8.87 | 8.86 | 8.87 | 8.86 | 8.87 | 8.87 |
| $^3\Sigma_u^-(\text{V}; \pi \to \pi^\star)$ | 9.78 | 9.68 | 9.68 | 9.67 | 9.68 | 9.67 | 9.68 | 9.67 | 9.67 | 9.67 |
| | Carbon monoxide | | | | | | | | | |
| $^1\Pi(\text{V}; n \to \pi^\star)$ | 8.57 | 8.49 | 8.47 | 8.46 | 8.47 | 8.45 | 8.47 | 8.45 | 8.45 | 8.45 |
| $^1\Sigma^-(\text{V}; \pi \to \pi^\star)$ | 10.12 | 9.99 | 9.99 | 9.98 | 9.99 | 9.98 | 9.99 | 9.98 | 9.98 | 9.98 |
| $^1\Delta(\text{V}; \pi \to \pi^\star)$ | 10.23 | 10.12 | 10.12 | 10.11 | 10.12 | 10.11 | 10.11 | 10.11 | 10.11 | 10.11 |
| $^1\Sigma^+(\text{R})$ | 10.92 | 10.94 | 10.90 | 10.91 | 10.72 | 10.72 | 10.72 | 10.72 | 10.85 | 10.74 |
| $^1\Sigma^+(\text{R})$ | 11.48 | 11.49 | 11.46 | 11.47 | 11.33 | 11.34 | 11.33 | 11.34 | 11.42 | 11.35 |
| $^1\Pi(\text{R})$ | 11.74 | 11.69 | 11.63 | 11.64 | 11.46 | 11.46 | 11.46 | 11.46 | 11.57 | 11.48 |
| $^3\Pi(\text{V}; n \to \pi^\star)$ | 6.31 | 6.30 | 6.30 | 6.29 | 6.30 | 6.29 | 6.30 | 6.29 | 6.29 | 6.29 |
| $^3\Sigma^+(\text{V}; \pi \to \pi^\star)$ | 8.45 | 8.45 | 8.48 | 8.47 | 8.48 | 8.47 | 8.48 | 8.47 | 8.48 | 8.48 |
| $^3\Delta(\text{V}; \pi \to \pi^\star)$ | 9.37 | 9.30 | 9.31 | 9.30 | 9.31 | 9.30 | 9.31 | 9.30 | 9.30 | 9.30 |
| $^3\Sigma^-(\text{V}; \pi \to \pi^\star)$ | 9.89 | 9.82 | 9.82 | 9.81 | 9.81 | 9.81 | 9.82 | 9.81 | 9.81 | 9.81 |
| $^3\Sigma^-(\text{R})$ | 10.39 | 10.45 | 10.44 | 10.45 | 10.33 | 10.33 | 10.33 | 10.34 | 10.42 | 10.35 |

### S1.3 Acetylene and ethylene

Table S3: CC3 vertical transition energies determined of acetylene (top) and ethylene (bottom) using various atomic basis sets. See caption of Table S1 for more details.

| | *aug*-cc-pVDZ | *aug*-cc-pVTZ | *aug*-cc-pVQZ | | d-*aug*-cc-pVQZ | | *aug*-cc-pV5Z | d-*aug*-cc-pV5Z |
|---|---|---|---|---|---|---|---|---|
| | FC | FC | FC | Full | FC | Full | Full | Full |
| | Acetylene | | | | | | | |
| $^1\Sigma_u^-(\pi \rightarrow \pi^\star)$ | 7.21 | 7.09 | 7.09 | 7.09 | 7.09 | 7.09 | 7.09 | 7.09 |
| $^1\Delta_u(\pi \rightarrow \pi^\star)$ | 7.51 | 7.42 | 7.41 | 7.42 | 7.41 | 7.42 | 7.42 | 7.42 |
| $^3\Sigma_u^+(\pi \rightarrow \pi^\star)$ | 5.48 | 5.50 | 5.53 | 5.52 | 5.53 | 5.52 | 5.53 | 5.53 |
| $^3\Delta_u(\pi \rightarrow \pi^\star)$ | 6.46 | 6.40 | 6.40 | 6.40 | 6.40 | 6.40 | 6.40 | 6.40 |
| $^3\Sigma_u^-(\pi \rightarrow \pi^\star)$ | 7.13 | 7.07 | 7.07 | 7.07 | 7.07 | 7.07 | 7.08 | 7.08 |
| $^1A_u[\mathrm{F}](\pi \rightarrow \pi^\star)$ | 3.70 | 3.64 | 3.63 | 3.63 | 3.63 | 3.63 | 3.63 | 3.63 |
| $^1A_2[\mathrm{F}](\pi \rightarrow \pi^\star)$ | 3.92 | 3.84 | 3.83 | 3.84 | 3.84 | 3.84 | 3.84 | 3.84 |
| | Ethylene | | | | | | | |
| $^1B_{3u}(\pi \rightarrow 3s)$ | 7.29 | 7.35 | 7.38 | 7.39 | 7.37 | 7.38 | 7.39 | 7.39 |
| $^1B_{1u}(\pi \rightarrow \pi^\star)$ | 7.94 | 7.91 | 7.90 | 7.91 | 7.90 | 7.93 | 7.91 | 7.90 |
| $^1B_{1g}(\pi \rightarrow 3p)$ | 7.97 | 8.03 | 8.04 | 8.05 | 8.03 | 8.04 | 8.05 | 8.05 |
| $^3B_{1u}(\pi \rightarrow \pi^\star)$ | 4.53 | 4.53 | 4.54 | 4.53 | 4.54 | 4.53 | 4.53 | 4.53 |
| $^3B_{3u}(\pi \rightarrow 3s)$ | 7.17 | 7.24 | 7.27 | 7.28 | 7.26 | 7.28 | 7.29 | 7.29 |
| $^3B_{1g}(\pi \rightarrow 3p)$ | 7.93 | 7.98 | 8.00 | 8.00 | 7.99 | 7.99 | 8.01 | 8.00 |

### S1.4 Formaldehyde, methanimine and thioformaldehyde

Table S4: CC3 vertical transition energies determined of formaldehyde (top), methanimine (center), and thioformaldehyde (bottom) using various atomic basis sets. See caption of Table S1 for more details.

| | *aug*-cc-pVDZ | *aug*-cc-pVTZ | *aug*-cc-pVQZ | | d-*aug*-cc-pVQZ | | *aug*-cc-pV5Z | d-*aug*-cc-pV5Z |
|---|---|---|---|---|---|---|---|---|
| | FC | FC | FC | Full | FC | Full | Full | Full |
| | Formaldehyde | | | | | | | |
| $^1A_2(n \to \pi^\star)$ | 4.00 | 3.97 | 3.97 | 3.96 | 3.97 | 3.96 | 3.96 | 3.96 |
| $^1B_2(n \to 3s)$ | 7.05 | 7.18 | 7.23 | 7.23 | 7.22 | 7.23 | 7.25 | 7.25 |
| $^1B_2(n \to 3p)$ | 8.02 | 8.07 | 8.10 | 8.11 | 8.05 | 8.06 | 8.10 | 8.08 |
| $^1A_1(n \to 3p)$ | 8.08 | 8.18 | 8.22 | 8.23 | 8.20 | 8.20 | 8.23 | 8.22 |
| $^1A_2(n \to 3p)$ | 8.65 | 8.64 | 8.60 | 8.61 | 8.44 | 8.45 | 8.54 | 8.47 |
| $^1B_1(\sigma \to \pi^\star)$ | 9.31 | 9.19 | 9.19 | 9.18 | 9.19 | 9.18 | 9.18 | 9.18 |
| $^1A_1(\pi \to \pi^\star)$ | 9.59 | 9.48 | 9.46 | 9.46 | 9.30 | 9.31 | 9.43 | 9.31 |
| $^3A_2(n \to \pi^\star)$ | 3.58 | 3.57 | 3.58 | 3.57 | 3.58 | 3.57 | 3.57 | 3.57 |
| $^3A_1(\pi \to \pi^\star)$ | 6.09 | 6.05 | 6.06 | 6.06 | 6.07 | 6.06 | 6.06 | 6.06 |
| $^3B_2(n \to 3s)$ | 6.91 | 7.03 | 7.08 | 7.09 | 7.08 | 7.09 | 7.11 | 7.11 |
| $^3B_2(n \to 3p)$ | 7.84 | 7.92 | 7.95 | 7.96 | 7.91 | 7.96 | 7.95 | 7.94 |
| $^3A_1(n \to 3p)$ | 7.97 | 8.08 | 8.12 | 8.12 | 8.10 | 8.11 | 8.13 | 8.13 |
| $^3B_1(n \to 3d)$ | 8.48 | 8.41 | 8.42 | 8.41 | 8.42 | 8.41 | 8.41 | 8.41 |
| $^1A''$[F]$(n \to \pi^\star)$ | 2.87 | 2.84 | 2.85 | 2.84 | 2.85 | 2.84 | 2.84 | 2.84 |
| | Methanimine | | | | | | | |
| $^1A''(n \to \pi^\star)$ | 5.26 | 5.20 | 5.20 | 5.18 | 5.20 | 5.18 | 5.18 | |
| $^3A''(n \to \pi^\star)$ | 4.63 | 4.61 | 4.62 | 4.60 | 4.62 | 4.60 | 4.60 | |
| | Thioformaldehyde | | | | | | | |
| $^1A_2(n \to \pi^\star)$ | 2.27 | 2.23 | 2.23 | 2.21 | 2.23 | 2.21 | 2.21 | |
| $^1B_2(n \to 4s)$ | 5.80 | 5.91 | 5.95 | 5.95 | 5.95 | 5.94 | 5.96 | |
| $^1A_1(\pi \to \pi^\star)$ | 6.62 | 6.48 | 6.46 | 6.45 | 6.45 | 6.45 | 6.43 | |
| $^3A_2(n \to \pi^\star)$ | 1.97 | 1.94 | 1.95 | 1.94 | 1.95 | 1.94 | 1.93 | |
| $^3A_1(\pi \to \pi^\star)$ | 3.43 | 3.38 | 3.40 | 3.39 | 3.40 | 3.39 | 3.39 | |
| $^3B_2(n \to 4s)$ | 5.64 | 5.72 | 5.75 | 5.75 | 5.75 | 5.74 | 5.75 | |
| $^1A_2$[F]$(n \to \pi^\star)$ | 2.00 | 1.97 | 1.98 | 1.96 | 1.97 | 1.96 | 1.95 | |

## S1.5 Larger compounds

Table S5: CC3 vertical transition energies of six compounds incorporating three non-hydrogen atoms. See caption of Table S1 for more details.

| Molecule state | | *aug*-cc-pVDZ FC | *aug*-cc-pVTZ FC | *aug*-cc-pVQZ FC | *aug*-cc-pVQZ Full | d-*aug*-cc-pVQZ Full |
|---|---|---|---|---|---|---|
| Acetaldehyde | $^1A''(n \to \pi^\star)$ | 4.34 | 4.31 | 4.32 | 4.31 | |
| | $^3A''(n \to \pi^\star)$ | 3.96 | 3.95 | 3.97 | 3.96 | |
| Cyclopropene | $^1B_1(\sigma \to \pi^\star)$ | 6.72 | 6.68 | 6.68 | 6.68 | |
| | $^1B_2(\pi \to \pi^\star)$ | 6.77 | 6.73 | 6.73 | 6.73 | |
| | $^3B_2(\pi \to \pi^\star)$ | 4.34 | 4.34 | 4.35 | 4.34 | |
| | $^3B_1(\sigma \to \pi^\star)$ | 6.43 | 6.40 | 6.41 | 6.40 | |
| Diazomethane | $^1A_2(\pi \to \pi^\star)$ | 3.10 | 3.07 | 3.07 | 3.06 | 3.06 |
| | $^1B_1(\pi \to 3s)$ | 5.32 | 5.45 | 5.49 | 5.51 | 5.50 |
| | $^1A_1(\pi \to \pi^\star)$ | 5.80 | 5.84 | 5.85 | 5.85 | 5.83 |
| | $^3A_2(\pi \to \pi^\star)$ | 2.84 | 2.83 | 2.82 | 2.82 | 2.83 |
| | $^3A_1(\pi \to \pi^\star)$ | 4.05 | 4.03 | 4.04 | 4.03 | 4.03 |
| | $^3B_1(\pi \to 3s)$ | 5.17 | 5.31 | 5.35 | 5.37 | 5.36 |
| | $^3A_1(\pi \to 3p)$ | 6.83 | 6.80 | 6.81 | 6.80 | 6.70 |
| | $^1A''[\mathrm{F}](\pi \to \pi^\star)$ | 0.68 | 0.68 | 0.68 | 0.67 | 0.67 |
| Formamide | $^1A''(n \to \pi^\star)$ | 5.71 | 5.66 | 5.66 | 5.64 | |
| | $^1A'(n \to 3s)$ | 6.65 | 6.74 | 6.78 | 6.79 | |
| | $^1A'(\pi \to \pi^\star)^a$ | 7.63 | 7.62 | 7.63 | 7.63 | |
| | $^1A'(n \to 3p)^a$ | 7.31 | 7.40 | 7.43 | 7.43 | |
| | $^3A''(n \to \pi^\star)$ | 5.42 | 5.38 | 5.39 | 5.37 | |
| | $^3A'(\pi \to \pi^\star)$ | 5.83 | 5.82 | 5.83 | 5.82 | |
| Ketene | $^1A_2(\pi \to \pi^\star)$ | 3.89 | 3.88 | 3.88 | 3.88 | 3.88 |
| | $^1B_1(n \to 3s)$ | 5.83 | 5.96 | 6.00 | 6.01 | 6.01 |
| | $^1A_2(\pi \to 3p)$ | 7.05 | 7.16 | 7.19 | 7.20 | 7.17 |
| | $^3A_2(n \to \pi^\star)$ | 3.79 | 3.78 | 3.79 | 3.78 | 3.78 |
| | $^3A_1(\pi \to \pi^\star)$ | 5.62 | 5.61 | 5.62 | 5.60 | 5.60 |
| | $^3B_1(n \to 3s)$ | 5.63 | 5.76 | 5.81 | 5.82 | 5.82 |
| | $^3A_2(\pi \to 3p)$ | 7.01 | 7.12 | 7.15 | 7.16 | 7.14 |
| | $^1A''[\mathrm{F}](\pi \to \pi^\star)$ | 1.00 | 1.00 | 1.00 | 1.00 | 1.00 |
| Nitrosomethane | $^1A''(n \to \pi^\star)$ | 2.00 | 1.96 | 1.96 | 1.96 | |
| | $^1A'(n, n \to \pi^\star, \pi^\star)$ | 5.75 | 5.76 | 5.74 | 5.73 | |
| | $^1A'(n \to 3s/3p)$ | 6.20 | 6.31 | 6.35 | 6.36 | |
| | $^3A''(n \to \pi^\star)$ | 1.13 | 1.14 | 1.15 | 1.14 | |
| | $^3A'(\pi \to \pi^\star)$ | 5.54 | 5.51 | 5.52 | 5.52 | |
| | $^1A''[\mathrm{F}](n \to \pi^\star)$ | 1.70 | 1.69 | 1.67 | 1.66 | |
| Streptocyanine-C1 | $^1B_2(\pi \to \pi^\star)$ | 7.14 | 7.13 | 7.13 | 7.12 | |
| | $^3B_2(\pi \to \pi^\star)$ | 5.48 | 5.48 | 5.49 | 5.48 | |

[a] Strong state mixing.

# S2 Geometries

Below are given the cartesian coordinates of the compounds investigated in this study. These are provided in atomic units (bohr) and they have been obtained at the CC3(full)/*aug*-cc-pVTZ level of theory.

## S2.1 Acetaldehyde

| | | | |
|---|---|---|---|
| C | -0.00234503 | 0.00000000 | 0.87125063 |
| C | -1.75847785 | 0.00000000 | -1.34973671 |
| O | 2.27947397 | 0.00000000 | 0.71968028 |
| H | -0.92904537 | 0.00000000 | 2.73929404 |
| H | -2.97955463 | 1.66046488 | -1.25209463 |
| H | -2.97955463 | -1.66046488 | -1.25209463 |
| H | -0.70043433 | 0.00000000 | -3.11066412 |

## S2.2 Acetylene

Ground state

| | | | |
|---|---|---|---|
| C | 0.00000000 | 0.00000000 | 1.14048351 |
| C | 0.00000000 | 0.00000000 | -1.14048351 |
| H | 0.00000000 | 0.00000000 | 3.14009043 |
| H | 0.00000000 | 0.00000000 | -3.14009043 |

*Trans* excited state ($^1A_u$ state in the $C_{2h}$ point group)

| | | | |
|---|---|---|---|
| C | 1.29567779 | 0.00000000 | -0.01846047 |
| C | -1.29567779 | 0.00000000 | 0.01846047 |
| H | 2.41938674 | 0.00000000 | 1.70881682 |
| H | -2.41938674 | 0.00000000 | -1.70881682 |

*Cis* excited state ($^1A_2$ state in the $C_{2v}$ point group)

| | | | |
|---|---|---|---|
| C | 0.00000000 | 1.26834508 | -0.11726146 |
| C | 0.00000000 | -1.26834508 | -0.11726146 |
| H | 0.00000000 | 2.67282325 | 1.39629264 |
| H | 0.00000000 | -2.67282325 | 1.39629264 |

## S2.3 Ammonia

| | | | |
|---|---|---|---|
| N | 0.12804615 | -0.00000000 | 0.00000000 |
| H | -0.59303935 | 0.88580079 | -1.53425197 |
| H | -0.59303935 | -1.77160157 | -0.00000000 |
| H | -0.59303935 | 0.88580079 | 1.53425197 |

## S2.4 Carbon monoxide

| | | | |
|---|---|---|---|
| C | 0.00000000 | 0.00000000 | -1.24942055 |
| O | 0.00000000 | 0.00000000 | 0.89266692 |

## S2.5 Cyclopropene

| | | | |
|---|---|---|---|
| C | 0.00000000 | 0.00000000 | -1.66820880 |
| C | 0.00000000 | 1.22523906 | 0.90681419 |
| C | 0.00000000 | -1.22523906 | 0.90681419 |
| H | 1.72255446 | 0.00000000 | -2.77881149 |
| H | -1.72255446 | 0.00000000 | -2.77881149 |
| H | 0.00000000 | 2.97844519 | 1.92076771 |
| H | 0.00000000 | -2.97844519 | 1.92076771 |

## S2.6 Diazomethane

Ground state

| | | | |
|---|---|---|---|
| C | 0.00000000 | 0.00000000 | -2.30830005 |
| N | 0.00000000 | 0.00000000 | 0.14457890 |
| N | 0.00000000 | 0.00000000 | 2.29923216 |
| H | 0.00000000 | 1.79875201 | -3.24272317 |
| H | 0.00000000 | -1.79875201 | -3.24272317 |

Excited state ($^1A$" state in the $C_s$ point group)

| | | | |
|---|---|---|---|
| C | 1.80206107 | 0.00000000 | -1.03389466 |
| N | -0.01743713 | 0.00000000 | 0.84742344 |
| N | -2.25203764 | 0.00000000 | 0.54034983 |
| H | 3.74280590 | 0.00000000 | -0.44375913 |
| H | 1.20115546 | 0.00000000 | -2.98380249 |

## S2.7 Dinitrogen

| | | | |
|---|---|---|---|
| N | 0.00000000 | 0.00000000 | 1.04008632 |
| N | 0.00000000 | 0.00000000 | -1.04008632 |

## S2.8 Ethylene

| | | | |
|---|---|---|---|
| C | 0.00000000 | 1.26026583 | 0.00000000 |
| C | 0.00000000 | -1.26026583 | 0.00000000 |
| H | 0.00000000 | 2.32345976 | 1.74287672 |
| H | 0.00000000 | -2.32345976 | 1.74287672 |
| H | 0.00000000 | 2.32345976 | -1.74287672 |
| H | 0.00000000 | -2.32345976 | -1.74287672 |

## S2.9 Formaldehyde

Ground state

| | | | |
|---|---|---|---|
| C | 0.00000000 | 0.00000000 | -1.13947666 |
| O | 0.00000000 | 0.00000000 | 1.14402883 |
| H | 0.00000000 | 1.76627623 | -2.23398653 |
| H | 0.00000000 | -1.76627623 | -2.23398653 |

Excited state ($^1A$" state in the $C_s$ point group)

| | | | |
|---|---|---|---|
| C | -0.09942705 | 0.00000000 | 1.27071070 |
| O | 0.01987299 | 0.00000000 | -1.23280536 |
| H | 0.42778855 | 1.76729629 | 2.18470884 |
| H | 0.42778855 | -1.76729629 | 2.18470884 |

## S2.10 Formamide

| | | | |
|---|---|---|---|
| C | 0.00183118 | 0.00000000 | 0.79313299 |
| O | 2.26817156 | 0.00000000 | 0.43918824 |
| N | -1.76886033 | 0.00000000 | -1.06219243 |
| H | -0.84133459 | 0.00000000 | 2.68872485 |
| H | -1.21254414 | 0.00000000 | -2.87596907 |
| H | -3.61627502 | 0.00000000 | -0.65031317 |

## S2.11 Hydrogen chloride

| | | | |
|---|---|---|---|
| Cl | 0.00000000 | 0.00000000 | -0.02489783 |
| H | 0.00000000 | 0.00000000 | 2.38483140 |

## S2.12 Hydrogen sulfide

| | | | |
|---|---|---|---|
| S | 0.00000000 | 0.00000000 | -0.50365086 |
| H | 0.00000000 | 1.81828105 | 1.25212288 |
| H | 0.00000000 | -1.81828105 | 1.25212288 |

## S2.13 Ketene

Ground state

| | | | |
|---|---|---|---|
| C | 0.00000000 | 0.00000000 | -2.44810151 |
| C | 0.00000000 | 0.00000000 | 0.03498545 |
| O | 0.00000000 | 0.00000000 | 2.23663914 |
| H | 0.00000000 | 1.77432079 | -3.43705988 |
| H | 0.00000000 | -1.77432079 | -3.43705988 |

Excited state ($^1A$" state in the $C_s$ point group)

| | | | |
|---|---|---|---|
| C | 2.04306304 | 0.00000000 | -0.93056721 |
| C | 0.00400918 | 0.00000000 | 0.83531393 |
| O | -2.23710378 | 0.00000000 | 0.46984584 |
| H | 1.63603518 | 0.00000000 | -2.93687368 |
| H | 3.96212800 | 0.00000000 | -0.26649149 |

## S2.14 Methanimine

| | | | |
|---|---|---|---|
| C | 0.10696646 | 0.00000000 | 1.11091130 |
| N | 0.10764012 | 0.00000000 | -1.29677742 |
| H | -1.59140953 | 0.00000000 | 2.27296652 |
| H | 1.90475160 | 0.00000000 | 2.09393982 |
| H | -1.69956184 | 0.00000000 | -1.96217482 |

## S2.15 Nitrosomethane

Ground state

| | | | |
|---|---|---|---|
| C | -1.78426612 | 0.00000000 | -1.07224050 |
| N | -0.00541753 | 0.00000000 | 1.08060391 |
| O | 2.18814985 | 0.00000000 | 0.43452135 |
| H | -0.77343975 | 0.00000000 | -2.86415606 |
| H | -2.97471478 | 1.66801808 | -0.86424584 |
| H | -2.97471478 | -1.66801808 | -0.86424584 |

Excited state ($^1A$" state in the $C_s$ point group)

| | | | |
|---|---|---|---|
| C | 1.86306273 | 0.00000000 | -1.06035094 |
| N | 0.00638693 | 0.00000000 | 1.02546010 |
| O | -2.26923072 | 0.00000000 | 0.47699489 |
| H | 3.72600129 | 0.00000000 | -0.21094854 |
| H | 1.58491147 | 1.68964774 | -2.20977225 |
| H | 1.58491147 | -1.68964774 | -2.20977225 |

## S2.16 Streptocyanine-C1

| | | | |
|---|---|---|---|
| C | 0.00000000 | 0.00000000 | 0.80488833 |
| N | 0.00000000 | 2.19423463 | -0.33580561 |
| N | 0.00000000 | -2.19423463 | -0.33580561 |
| H | 0.00000000 | 0.00000000 | 2.84436959 |
| H | 0.00000000 | 2.36978315 | -2.23371976 |
| H | 0.00000000 | -2.36978315 | -2.23371976 |
| H | 0.00000000 | 3.79412648 | 0.69399206 |
| H | 0.00000000 | -3.79412648 | 0.69399206 |

## S2.17 Thioformaldehyde

Ground state

| | | | |
|---|---|---|---|
| C | 0.00000000 | 0.00000000 | -2.08677304 |
| S | 0.00000000 | 0.00000000 | 0.97251194 |
| H | 0.00000000 | 1.73657773 | -3.17013507 |
| H | 0.00000000 | -1.73657773 | -3.17013507 |

Excited state ($^1A_2$ state in the $C_{2v}$ point group)

| | | | |
|---|---|---|---|
| C | 0.00000000 | 0.00000000 | -2.20256705 |
| S | 0.00000000 | 0.00000000 | 1.02717172 |
| H | 0.00000000 | 1.76634191 | -3.21909384 |
| H | 0.00000000 | -1.76634191 | -3.21909384 |

## S2.18 Water

| | | | |
|---|---|---|---|
| O | 0.00000000 | 0.00000000 | -0.13209669 |
| H | 0.00000000 | 1.43152878 | 0.97970006 |
| H | 0.00000000 | -1.43152878 | 0.97970006 |

## S3 Benchmark

Table S6: Comparisons between the TBE(FC)/*aug*-cc-pVTZ benchmark (see Table 6) and the results obtained with various computational approaches using the same basis set and approximation. STEOM stands for STEOM-CCSD and CC(3) for CCSDR(3).

| Compound | State | TBE | CIS(D) | CIS($D_\infty$) | CC2 | STEOM | CCSD | CC(3) | CCSDT-3 | CC3 | CCSDT | CCSDTQ | ADC(2) | ADC(3) |
|---|---|---|---|---|---|---|---|---|---|---|---|---|---|---|
| Acetaldehyde | $^1A''(\mathrm{V}; n \to \pi^\star)$ | 4.31 | 4.36 | 4.24 | 4.41 | 4.25 | 4.36 | 4.31 | 4.32 | 4.31 | 4.29 | | 4.24 | 4.29 |
| | $^3A''(\mathrm{V}; n \to \pi^\star)$ | 3.97 | 3.96 | 3.83 | 3.98 | 3.95 | 3.95 | | | 3.95 | 3.94 | | 3.83 | 3.89 |
| Acetylene | $^1\Sigma_u^-(\mathrm{V}; \pi \to \pi^\star)$ | 7.10 | 7.28 | 7.24 | 7.26 | 7.08 | 7.15 | 7.09 | 7.09 | 7.09 | 7.09 | 7.09[a] | 7.24 | 6.72 |
| | $^1\Delta_u(\mathrm{V}; \pi \to \pi^\star)$ | 7.44 | 7.62 | 7.56 | 7.59 | 7.42 | 7.48 | 7.43 | 7.42 | 7.42 | 7.43 | 7.43[a] | 7.56 | 7.06 |
| | $^3\Sigma_u^+(\mathrm{V}; \pi \to \pi^\star)$ | 5.53 | 5.79 | 5.75 | 5.76 | 5.20 | 5.45 | | | 5.50 | 5.51 | 5.52[a] | 5.75 | 5.24 |
| | $^3\Delta_u(\mathrm{V}; \pi \to \pi^\star)$ | 6.40 | 6.62 | 6.57 | 6.60 | 6.13 | 6.41 | | | 6.40 | 6.39 | 6.39[a] | 6.57 | 6.06 |
| | $^3\Sigma_u^-(\mathrm{V}; \pi \to \pi^\star)$ | 7.08 | 7.31 | 7.27 | 7.29 | 6.84 | 7.12 | | | 7.07 | 7.08[b] | 7.08[c] | 7.27 | 6.72 |
| | $^1A_u[\mathrm{F}](\mathrm{V}; \pi \to \pi^\star)$ | 3.64 | 3.85 | 3.78 | 3.94 | 3.65 | 3.70 | 3.66 | 3.64 | 3.64 | 3.66 | 3.64[a] | 3.78 | 2.85 |
| | $^1A_2[\mathrm{F}](\mathrm{V}; \pi \to \pi^\star)$ | 3.85 | 4.06 | 3.99 | 4.11 | 3.85 | 3.92 | 3.85 | 3.84 | 3.84 | 3.86 | 3.85[a] | 3.99 | 3.08 |
| Ammonia | $^1A_2(\mathrm{R}; n \to 3s)$ | 6.59 | 6.37 | 6.40 | 6.39 | 6.55 | 6.60 | 6.57 | 6.58 | 6.57 | 6.57 | 6.59 | 6.40 | 6.63 |
| | $^1E(\mathrm{R}; n \to 3p)$ | 8.16 | 7.86 | 7.87 | 7.85 | 8.14 | 8.15 | 8.15 | 8.15 | 8.15 | 8.14 | 8.16 | 7.87 | 8.21 |
| | $^1A_1(\mathrm{R}; n \to 3p)$ | 9.33 | 9.04 | 9.05 | 9.05 | 9.33 | 9.33 | 9.32 | 9.32 | 9.32 | 9.31 | 9.34[a] | 9.05 | 9.38 |
| | $^1A_2(\mathrm{R}; n \to 4s)$ | 9.96 | 9.59 | 9.67 | 9.65 | 9.98 | 9.95 | 9.94 | 9.95 | 9.95 | 9.94 | 9.96[a] | 9.67 | 10.00 |
| | $^3A_2(\mathrm{R}; n \to 3s)$ | 6.31 | 6.18 | 6.16 | 6.14 | 6.31 | 6.30 | | | 6.29 | 6.29 | 6.30 | 6.16 | 6.31 |
| Carbon monoxyde | $^1\Pi(\mathrm{V}; n \to \pi^\star)$ | 8.49 | 8.78 | 8.69 | 8.64 | 8.55 | 8.59 | 8.52 | 8.51 | 8.49 | 8.49 | 8.48 | 8.69 | 8.24 |
| | $^1\Sigma^-(\mathrm{V}; \pi \to \pi^\star)$ | 9.92 | 10.13 | 10.03 | 10.30 | 9.90 | 9.99 | 9.98 | 9.98 | 9.99 | 9.94 | 9.93 | 10.03 | 9.73 |
| | $^1\Delta(\mathrm{V}; \pi \to \pi^\star)$ | 10.06 | 10.41 | 10.30 | 10.60 | 10.07 | 10.12 | 10.12 | 10.11 | 10.12 | 10.08 | 10.07 | 10.30 | 9.82 |
| | $^1\Sigma^+(\mathrm{R})$ | 10.95 | 11.48 | 11.32 | 11.11 | 11.14 | 11.22 | 10.99 | 11.02 | 10.94 | 10.99 | 10.96 | 11.32 | 10.79 |
| | $^1\Sigma^+(\mathrm{R})$ | 11.52 | 11.71 | 11.83 | 11.63 | 11.75 | 11.75 | 11.53 | 11.55 | 11.49 | 11.54 | 11.52 | 11.83 | 11.33 |
| | $^1\Pi(\mathrm{R})$ | 11.72 | 12.06 | 12.03 | 11.83 | 12.00 | 11.96 | 11.73 | 11.76 | 11.69 | 11.74 | 11.72 | 12.03 | 11.56 |
| | $^3\Pi(\mathrm{V}; n \to \pi^\star)$ | 6.28 | 6.51 | 6.45 | 6.42 | 6.32 | 6.36 | | | 6.30 | 6.30 | 6.28 | 6.45 | 5.97 |
| | $^3\Sigma^+(\mathrm{V}; \pi \to \pi^\star)$ | 8.45 | 8.63 | 8.54 | 8.72 | 8.37 | 8.34 | | | 8.45 | 8.42 | 8.44 | 8.54 | 8.21 |
| | $^3\Delta(\mathrm{V}; \pi \to \pi^\star)$ | 9.27 | 9.44 | 9.33 | 9.56 | 9.21 | 9.23 | | | 9.30 | 9.26 | 9.26 | 9.33 | 9.03 |
| | $^3\Sigma^-(\mathrm{V}; \pi \to \pi^\star)$ | 9.80 | 10.10 | 10.01 | 10.27 | 9.83 | 9.81 | | | 9.82 | | | 10.01 | 9.53 |
| | $^3\Sigma^+(\mathrm{R})$ | 10.47 | 10.98 | 10.83 | 10.60 | 10.73 | 10.71 | | | 10.45 | 10.50 | 10.48 | 10.83 | 10.29 |
| Cyclopropene | $^1B_1(\mathrm{V}; \sigma \to \pi^\star)$ | 6.68 | 6.90 | 6.75 | 6.73 | | 6.76 | 6.68 | 6.70 | 6.68 | 6.68 | | 6.75 | 6.56 |
| | $^1B_2(\mathrm{V}; \pi \to \pi^\star)$ | 6.79 | 6.90 | 6.86 | 6.78 | 6.94 | 6.86 | 6.73 | 6.76 | 6.73 | 6.75 | | 6.86 | 6.56 |
| | $^3B_2(\mathrm{V}; \pi \to \pi^\star)$ | 4.38 | 4.55 | 4.45 | 4.46 | 4.36 | 4.30 | | | 4.34 | 4.35[b] | | 4.45 | 4.09 |
| | $^3B_1(\mathrm{V}; \sigma \to \pi^\star)$ | 6.45 | 6.49 | 6.45 | 6.44 | 6.57 | 6.46 | | | 6.40 | 6.40[b] | | 6.45 | 6.26 |
| Diazomethane | $^1A_2(\mathrm{V}; \pi \to \pi^\star)$ | 3.14 | 3.55 | 3.34 | 3.37 | 3.20 | 3.19 | 3.12 | 3.10 | 3.07 | 3.07 | | 3.34 | 2.74 |
| | $^1B_1(\mathrm{R}; \pi \to 3s)$ | 5.54 | 5.65 | 5.63 | 5.53 | 5.57 | 5.57 | 5.48 | 5.47 | 5.45 | 5.48 | | 5.63 | 5.23 |
| | $^1A_1(\mathrm{V}; \pi \to \pi^\star)$ | 5.90 | 6.03 | 5.97 | 6.00 | 5.75 | 5.94 | 5.87 | 5.86 | 5.84 | 5.86 | | 5.97 | 5.48 |
| | $^3A_2(\mathrm{V}; \pi \to \pi^\star)$ | 2.79 | 3.21 | 3.00 | 3.08 | 2.85 | 3.19 | | | 2.83 | 2.82 | | 3.01 | 2.44 |
| | $^3A_1(\mathrm{V}; \pi \to \pi^\star)$ | 4.05 | 4.28 | 4.20 | 4.25 | 3.91 | 3.95 | | | 4.03 | 4.02 | | 4.20 | 3.64 |

Continued on next page

| Compound | State | TBE | CIS(D) | CIS($D_\infty$) | CC2 | STEOM | CCSD | CC(3) | CCSDT-3 | CC3 | CCSDT | CCSDTQ | ADC(2) | ADC(3) |
|---|---|---|---|---|---|---|---|---|---|---|---|---|---|---|
| | $^3B_1$(R; $\pi \to 3s$) | 5.35 | 5.53 | 5.50 | 5.53 | 5.43 | 5.42 | | | 5.31 | 5.34 | | 5.50 | 5.08 |
| | $^3A_1$(R; $\pi \to 3p$) | 6.82 | 7.37 | 7.09 | 7.04 | | 6.85 | | | 6.80 | 6.80[b] | | 7.09 | 6.36 |
| | $^1A''$[F](V; $\pi \to \pi^\star$) | 0.71 | 1.06 | 0.80 | 0.90 | 0.88 | 0.81 | 0.73 | 0.70 | 0.68 | 0.67 | | 0.81 | 0.24 |
| Dinitrogen | $^1\Pi_g$(V; $n \to \pi^\star$) | 9.34 | 9.66 | 9.48 | 9.44 | 9.37 | 9.41 | 9.36 | 9.35 | 9.34 | 9.33 | 9.32 | 9.48 | 9.16 |
| | $^1\Sigma_u^-$(V; $\pi \to \pi^\star$) | 9.88 | 10.31 | 10.26 | 10.32 | 10.09 | 10.00 | 9.90 | 9.89 | 9.88 | 9.89 | 9.88 | 10.26 | 9.33 |
| | $^1\Delta_u$(V; $\pi \to \pi^\star$) | 10.29 | 10.85 | 10.79 | 10.86 | 10.56 | 10.44 | 10.33 | 10.31 | 10.29 | 10.30 | 10.29[a] | 10.79 | 9.74 |
| | $^1\Sigma_g^+$(R) | 12.98 | 13.67 | 12.99 | 12.83 | 13.13 | 13.15 | 13.04 | 13.06 | 13.01 | 13.00 | 12.97 | 12.99 | 13.01 |
| | $^1\Pi_u$(R) | 13.03 | 13.64 | 13.33 | 13.15 | 13.43 | 13.43 | 13.28 | 13.27 | 13.22 | 13.14 | 13.09 | 13.32 | 12.98 |
| | $^1\Sigma_u^+$(R) | 13.09 | 13.75 | 13.07 | 12.89 | 13.22 | 13.26 | 13.14 | 13.16 | 13.12 | 13.12 | 13.09 | 13.07 | 13.09 |
| | $^1\Pi_u$(R) | 13.46 | 14.52 | 13.99 | 13.96 | 13.73 | 13.67 | 13.52 | | 13.49 | 13.45 | 13.42 | 14.00 | 13.40 |
| | $^3\Sigma_u^+$(V; $\pi \to \pi^\star$) | 7.70 | 8.20 | 8.15 | 8.19 | 7.70 | 7.66 | | | 7.68 | 7.69 | 7.70 | 8.15 | 7.25 |
| | $^3\Pi_g$(V; $n \to \pi^\star$) | 8.01 | 8.33 | 8.20 | 8.19 | 8.16 | 8.09 | | | 8.04 | 8.03 | 8.02 | 8.20 | 7.77 |
| | $^3\Delta_u$(V; $\pi \to \pi^\star$) | 8.87 | 9.30 | 9.25 | 9.30 | 8.94 | 8.91 | | | 8.87 | 8.87 | 8.87 | 9.25 | 8.36 |
| | $^3\Sigma_u^-$(V; $\pi \to \pi^\star$) | 9.66 | 10.29 | 10.23 | 10.29 | 9.90 | 9.83 | | | 9.68 | 9.68 | 9.66 | 10.23 | 9.14 |
| Ethylene | $^1B_{3u}$(R; $\pi \to 3s$) | 7.40 | 7.35 | 7.34 | 7.29 | 7.42 | 7.42 | 7.35 | 7.36 | 7.35 | 7.37 | 7.38[a] | 7.34 | 7.17 |
| | $^1B_{1u}$(V; $\pi \to \pi^\star$) | 7.91 | 7.95 | 7.92 | 7.92 | | 8.02 | 7.89 | 7.92 | 7.91 | 7.92 | 7.91[a] | 7.91 | 7.69 |
| | $^1B_{1g}$(R; $\pi \to 3p$) | 8.07 | 8.01 | 7.99 | 7.95 | 8.10 | 8.08 | 8.02 | 8.03 | 8.03 | 8.04 | 8.05[a] | 7.99 | 7.84 |
| | $^3B_{1u}$(V; $\pi \to \pi^\star$) | 4.54 | 4.62 | 4.59 | 4.59 | 4.36 | 4.46 | | | 4.53 | 4.53 | 4.53[a] | 4.59 | 4.28 |
| | $^3B_{3u}$(R; $\pi \to 3s$) | 7.23 | 7.26 | 7.23 | 7.19 | 7.31 | 7.29 | | | 7.24 | 7.25 | 7.25[a] | 7.23 | 7.05 |
| | $^3B_{1g}$(R; $\pi \to 3p$) | 7.98 | 7.97 | 7.95 | 7.91 | 8.08 | 8.03 | | | 7.98 | 7.99 | 7.99[a] | 7.95 | 7.80 |
| Formaldehyde | $^1A_2$(V; $n \to \pi^\star$) | 3.98 | 4.04 | 3.92 | 4.07 | 3.91 | 4.01 | 3.97 | 3.98 | 3.97 | 3.95 | 3.96[a] | 3.92 | 3.90 |
| | $^1B_2$(R; $n \to 3s$) | 7.23 | 6.64 | 6.50 | 6.56 | 7.19 | 7.23 | 7.18 | 7.21 | 7.18 | 7.16 | 7.21[a] | 6.50 | 7.62 |
| | $^1B_2$(R; $n \to 3p$) | 8.13 | 7.56 | 7.53 | 7.57 | 8.05 | 8.12 | 8.08 | 8.11 | 8.07 | 8.07 | 8.11[a] | 7.53 | 8.45 |
| | $^1A_1$(R; $n \to 3p$) | 8.23 | 8.16 | 7.47 | 7.52 | 8.18 | 8.21 | 8.17 | 8.21 | 8.18 | 8.16 | 8.21[a] | 7.47 | 8.61 |
| | $^1A_2$(R; $n \to 3p$) | 8.67 | 8.04 | 7.99 | 8.04 | 8.68 | 8.65 | 8.63 | 8.66 | 8.64 | 8.61 | 8.66[a] | 7.99 | 9.02 |
| | $^1B_1$(V; $\sigma \to \pi^\star$) | 9.22 | 9.38 | 9.17 | 9.32 | 9.08 | 9.28 | 9.20 | 9.20 | 9.19 | 9.17 | 9.18[a] | 9.17 | 9.17 |
| | $^1A_1$(V; $\pi \to \pi^\star$) | 9.43 | 9.08 | 9.46 | 9.54 | | 9.67 | 9.51 | 9.51 | 9.48 | 9.49 | 9.44[a] | 9.46 | 9.05 |
| | $^3A_2$(V; $n \to \pi^\star$) | 3.58 | 3.58 | 3.46 | 3.59 | 3.54 | 3.56 | | | 3.57 | 3.56 | 3.57[a] | 3.46 | 3.48 |
| | $^3A_1$(V; $\pi \to \pi^\star$) | 6.06 | 6.27 | 6.20 | 6.30 | 5.89 | 5.97 | | | 6.05 | 6.05 | 6.06[a] | 6.20 | 5.71 |
| | $^3B_2$(R; $n \to 3s$) | 7.06 | 6.66 | 6.39 | 6.44 | 7.07 | 7.08 | | | 7.03 | 7.02 | 7.07[a] | 6.39 | 7.44 |
| | $^3B_2$(R; $n \to 3p$) | 7.94 | 7.52 | 7.41 | 7.45 | 7.98 | 7.94 | | | 7.92 | 7.90 | 7.94[a] | 7.41 | 8.23 |
| | $^3A_1$(R; $n \to 3p$) | 8.10 | 7.68 | 7.40 | 7.44 | 8.15 | 8.09 | | | 8.08 | 8.06 | 8.11[a] | 7.40 | 8.46 |
| | $^3B_1$(R; $n \to 3d$) | 8.42 | 8.57 | 8.39 | 8.52 | 8.36 | 8.43 | | | 8.41 | 8.40 | 8.41[a] | 8.39 | 8.32 |
| | $^1A$"[F](V; $n \to \pi^\star$) | 2.80 | 2.90 | 2.71 | 2.97 | 2.81 | 2.93 | 2.86 | 2.86 | 2.84 | 2.82 | 2.84[a] | 2.71 | 2.77 |
| Formamide | $^1A''$V; ($n \to \pi^\star$) | 5.65 | 5.58 | 5.45 | 5.69 | 5.72 | 5.69 | 5.66 | 5.67 | 5.66 | 5.63[b] | | 5.45 | 5.75 |
| | $^1A'$(R; $n \to 3s$) | 6.77 | 6.82[d] | 6.26[d] | 6.31[d] | 6.94 | 6.99 | 6.83 | 6.83 | 6.74 | 6.74 | | 6.26[d] | 7.20 |
| | $^1A'$(V; $\pi \to \pi^\star$) | 7.63 | 6.84[d] | 7.39[d] | 7.55[d] | | 7.55[d] | 7.44 | 7.68[d] | 7.62[d] | 7.61[b] | | 7.39[d] | 7.80[d] |
| | $^1A'$(R; $n \to 3p$) | 7.38 | 6.89[d] | 6.83[d] | 6.89[d] | | 7.78[d] | 7.65 | 7.46[d] | 7.40[d] | 7.38[b] | | 6.83[d] | 8.12[d] |
| | $^3A''$(V; $n \to \pi^\star$) | 5.38 | 5.31 | 5.15 | 5.36 | 5.29 | 5.36 | | | 5.38 | 5.35[b] | | 5.15 | 5.42 |

Continued on next page

| Compound | State | TBE | CIS(D) | CIS(D$_\infty$) | CC2 | STEOM | CCSD | CC(3) | CCSDT-3 | CC3 | CCSDT | CCSDTQ | ADC(2) | ADC(3) |
|---|---|---|---|---|---|---|---|---|---|---|---|---|---|---|
| | $^3A'(\text{V};\pi \to \pi^\star)$ | 5.81 | 6.07 | 5.88 | 5.99 | 5.74 | 5.77 | | | 5.82 | 5.80$^b$ | | 5.88 | 5.63 |
| Hydrogen chloride | $^1\Pi(\text{CT})$ | 7.84 | 7.98 | 7.97 | 7.96 | 7.91 | 7.91 | 7.84 | 7.85 | 7.84 | 7.83 | 7.84 | 7.97 | 7.79 |
| Hydrogen sulfide | $^1A_2(\text{R};n \to 4p)$ | 6.18 | 6.38 | 6.37 | 6.35 | 6.23 | 6.25 | 6.25 | 6.23 | 6.19 | 6.18 | 6.18 | 6.37 | 6.05 |
| | $^1B_1(\text{R};n \to 4s)$ | 6.24 | 6.33 | 6.34 | 6.30 | 6.31 | 6.29 | 6.29 | 6.28 | 6.24 | 6.24 | 6.24 | 6.34 | 6.18 |
| | $^3A_2(\text{R};n \to 4p)$ | 5.81 | 5.94 | 5.91 | 5.91 | 5.96 | 5.85 | | | 5.82 | 5.81 | 5.81 | 5.91 | 5.67 |
| | $^3B_1(\text{R};n \to 4s)$ | 5.88 | 5.99 | 5.96 | 5.94 | 5.98 | 5.92 | | | 5.88 | 5.88 | 5.88 | 5.96 | 5.81 |
| Ketene | $^1A_2(\text{V};\pi \to \pi^\star)$ | 3.86 | 4.18 | 4.11 | 4.17 | 3.84 | 3.97 | 3.92 | 3.90 | 3.88 | 3.87 | | 4.11 | 3.67 |
| | $^1B_1(\text{R};n \to 3s)$ | 6.01 | 6.09 | 6.03 | 5.94 | 6.08 | 6.09 | 5.99 | 5.99 | 5.96 | 5.99 | | 6.03 | 5.87 |
| | $^1A_2(\text{R};\pi \to 3p)$ | 7.18 | 7.25 | 7.18 | 7.09 | 7.29 | 7.29 | 7.19 | 7.20 | 7.16 | 7.20 | | 7.18 | 7.07 |
| | $^3A_2(\text{V};n \to \pi^\star)$ | 3.77 | 4.00 | 3.92 | 3.98 | 3.82 | 3.83 | | | 3.78 | 3.78 | | 3.92 | 3.56 |
| | $^3A_1(\text{V};\pi \to \pi^\star)$ | 5.61 | 5.79 | 5.67 | 5.72 | 5.53 | 5.55 | | | 5.61 | 5.60 | | 5.67 | 5.39 |
| | $^3B_1(\text{R};n \to 3s)$ | 5.79 | 5.94 | 5.85 | 5.77 | 5.91 | 5.89 | | | 5.76 | 5.80 | | 5.85 | 5.67 |
| | $^3A_2(\text{R};\pi \to 3p)$ | 7.12 | 7.24 | 7.15 | 7.06 | 7.32 | 7.25 | | | 7.12 | 7.17 | | 7.15 | 7.03 |
| | $^1A''[\text{F}](\text{V};\pi \to \pi^\star)$ | 1.00 | 1.28 | 1.20 | 1.26 | 1.03 | 1.13 | 1.06 | 1.03 | 1.00 | 1.00 | | 1.19 | 0.67 |
| Methanimine | $^1A''(\text{V};n \to \pi^\star)$ | 5.23 | 5.38 | 5.29 | 5.32 | 5.20 | 5.28 | 5.20 | 5.22 | 5.20 | 5.19 | 5.20$^a$ | 5.29 | 5.05 |
| | $^3A''(\text{V};n \to \pi^\star)$ | 4.65 | 4.71 | 4.61 | 4.65 | 4.62 | 4.63 | | | 4.61 | 4.61 | 4.61$^a$ | 4.61 | 4.44 |
| Nitrosomethane | $^1A''(\text{V};n \to \pi^\star)$ | 1.96 | 2.03 | 1.88 | 1.98 | 1.80 | 1.98 | 1.96 | 1.96 | 1.96 | 1.95 | | 1.88 | 1.72 |
| | $^1A'(\text{V};n,n \to \pi^\star,\pi^\star)$ | 4.72 | | | | | | | 6.02 | 5.76 | 5.29 | | | 3.00 |
| | $^1A'(\text{R};n \to 3s/3p)$ | 6.40 | 5.89 | 5.86 | 5.84 | 6.51 | 6.43 | 6.33 | 6.38 | 6.31 | 6.30 | | 5.86 | 6.48 |
| | $^3A''(\text{V};n \to \pi^\star)$ | 1.16 | 1.18 | 1.03 | 1.12 | 0.99 | 1.11 | | | 1.14 | 1.13 | | 1.03 | 0.84 |
| | $^3A'(\text{V};\pi \to \pi^\star)$ | 5.60 | 5.89 | 5.75 | 5.74 | 5.04 | 5.43 | | | 5.51 | 5.51$^b$ | | 5.75 | 5.04 |
| | $^1A''[\text{F}](\text{V};n \to \pi^\star)$ | 1.67 | 1.73 | 1.55 | 1.68 | 1.49 | 1.68 | 1.67 | 1.67 | 1.69 | 1.66 | | 1.55 | 1.40 |
| Streptocyanine | $^1B_2(\text{V};\pi \to \pi^\star)$ | 7.13 | 6.99 | 7.00 | 7.20 | 6.76 | 7.24 | 7.12 | 7.16 | 7.13 | 7.11 | | 7.00 | 7.16 |
| | $^3B_2(\text{V};\pi \to \pi^\star)$ | 5.47 | 5.61 | 5.55 | 5.60 | 5.40 | 5.45 | | | 5.48 | 5.47 | | 5.55 | 5.33 |
| Thioformaldehyde | $^1A_2(\text{V};n \to \pi^\star)$ | 2.22 | 2.30 | 2.24 | 2.34 | 2.17 | 2.29 | 2.22 | 2.24 | 2.23 | 2.21 | 2.22$^a$ | 2.24 | 2.05 |
| | $^1B_2(\text{R};n \to 4s)$ | 5.96 | 5.87 | 5.80 | 5.82 | 5.92 | 5.97 | 5.90 | 5.94 | 5.91 | 5.89 | 5.91$^a$ | 5.80 | 5.94 |
| | $^1A_1(\text{V};\pi \to \pi^\star)$ | 6.38 | 6.65 | 6.57 | 6.71 | 6.48 | 6.63 | 6.50 | 6.51 | 6.48 | 6.47 | 6.38$^a$ | 6.57 | 5.98 |
| | $^3A_2(\text{V};n \to \pi^\star)$ | 1.94 | 1.94 | 1.86 | 1.94 | 1.91 | 1.95 | | | 1.94 | 1.93 | 1.93$^a$ | 1.86 | 1.77 |
| | $^3A_1(\text{V};\pi \to \pi^\star)$ | 3.43 | 3.49 | 3.45 | 3.48 | 3.18 | 3.28 | | | 3.38 | 3.38 | 3.39$^a$ | 3.45 | 3.07 |
| | $^3B_2(\text{R};n \to 4s)$ | 5.72 | 5.78 | 5.62 | 5.64 | 5.71 | 5.76 | | | 5.72 | 5.71 | 5.73$^a$ | 5.62 | 5.71 |
| | $^1A_2[\text{F}](\text{V};n \to \pi^\star)$ | 1.95 | 2.00 | 1.92 | 2.09 | 1.92 | 2.05 | 1.97 | 1.98 | 1.97 | 1.98 | 1.96$^a$ | 1.92 | 1.80 |
| Water | $^1B_1(\text{R};n \to 3s)$ | 7.62 | 7.17 | 7.18 | 7.23 | 7.56 | 7.60 | 7.60 | 7.61 | 7.65 | 7.65 | 7.62 | 7.18 | 7.84 |
| | $^1A_2(\text{R};n \to 3p)$ | 9.41 | 8.92 | 8.84 | 8.89 | 9.37 | 9.36 | 9.38 | 9.38 | 9.43 | 9.42 | 9.40 | 8.84 | 9.63 |
| | $^1A_1(\text{R};n \to 3s)$ | 9.99 | 9.52 | 9.52 | 9.58 | 9.92 | 9.96 | 9.96 | 9.97 | 10.00 | 9.98 | 9.98 | 9.52 | 10.22 |
| | $^3B_1(\text{R};n \to 3s)$ | 7.25 | 6.92 | 6.86 | 6.91 | 7.24 | 7.20 | | | 7.28 | 7.28 | 7.24 | 6.86 | 7.41 |
| | $^3A_2(\text{R};n \to 3p)$ | 9.24 | 8.91 | 8.72 | 8.77 | 9.21 | 9.20 | | | 9.26 | 9.25 | 9.23 | 8.72 | 9.43 |
| | $^3A_1(\text{R};n \to 3s)$ | 9.54 | 9.30 | 9.15 | 9.20 | 9.51 | 9.49 | | | 9.56 | 9.54 | 9.53 | 9.15 | 9.70 |

[a]CCSDTQ/*aug*-cc-pVDZ value corrected with the difference between CCSDT/*aug*-cc-pVTZ and CCSDT/*aug*-cc-pVDZ values; [b]CCSDT/*aug*-cc-pVDZ

value corrected with the difference between CC3/*aug*-cc-pVTZ and CC3/*aug*-cc-pVDZ values; [c]CCSDTQ/*aug*-cc-pVDZ value corrected with the difference between CC3/*aug*-cc-pVTZ and CC3/*aug*-cc-pVDZ values; [d]Strong state mixing.

# S4 Additional statistical analyses

Table S7: Mean signed and absolute errors for different subsets of electronic transitions. $\%T_1$ indicates the single excitation character as given by CC3, see Table 6 in the body of the paper. All values are in eV.

| Type | | CIS(D) | CIS($D_\infty$) | CC2 | STEOM | CCSD | CC(3) | CCSDT-3 | CC3 | CCSDT | CCSDTQ | ADC(2) | ADC(3) |
|---|---|---|---|---|---|---|---|---|---|---|---|---|---|
| Singlet | MSE | 0.08 | -0.02 | 0.01 | 0.03 | 0.08 | 0.01 | 0.01 | 0.00 | -0.01 | 0.00 | -0.02 | -0.14 |
| | MAE | 0.28 | 0.22 | 0.23 | 0.09 | 0.08 | 0.04 | 0.03 | 0.03 | 0.03 | 0.01 | 0.22 | 0.22 |
| Triplet | MSE | 0.12 | 0.01 | 0.06 | -0.02 | 0.01 | | | -0.01 | -0.01 | 0.00 | 0.01 | -0.18 |
| | MAE | 0.22 | 0.19 | 0.20 | 0.11 | 0.07 | | | 0.02 | 0.02 | 0.01 | 0.19 | 0.25 |
| Valence | MSE | 0.18 | 0.09 | 0.17 | -0.03 | 0.04 | 0.01 | 0.01 | 0.00 | -0.01 | -0.01 | 0.09 | -0.27 |
| | MAE | 0.20 | 0.15 | 0.18 | 0.10 | 0.08 | 0.03 | 0.03 | 0.02 | 0.02 | 0.01 | 0.15 | 0.28 |
| Rydberg | MSE | -0.01 | -0.14 | -0.17 | 0.06 | 0.06 | 0.00 | 0.01 | -0.01 | -0.01 | 0.00 | -0.14 | 0.01 |
| | MAE | 0.32 | 0.29 | 0.26 | 0.09 | 0.08 | 0.05 | 0.04 | 0.03 | 0.03 | 0.01 | 0.29 | 0.17 |
| $n \rightarrow \pi^\star$ | MSE | 0.11 | -0.01 | 0.08 | -0.02 | 0.04 | 0.01 | 0.02 | 0.00 | -0.01 | 0.00 | -0.01 | -0.16 |
| | MAE | 0.12 | 0.12 | 0.09 | 0.07 | 0.06 | 0.02 | 0.02 | 0.01 | 0.02 | 0.02 | 0.12 | 0.18 |
| $\pi \rightarrow \pi^\star$ | MSE | 0.23 | 0.16 | 0.24 | -0.05 | 0.03 | 0.01 | 0.01 | 0.00 | -0.01 | 0.00 | 0.16 | -0.35 |
| | MAE | 0.26 | 0.17 | 0.24 | 0.13 | 0.09 | 0.04 | 0.03 | 0.03 | 0.02 | 0.01 | 0.17 | 0.36 |
| $\%T_1 > 95\%$ | MSE | 0.13 | 0.03 | 0.07 | -0.01 | 0.02 | -0.01 | -0.01 | -0.01 | -0.01 | 0.00 | 0.03 | -0.22 |
| | MAE | 0.22 | 0.19 | 0.21 | 0.10 | 0.07 | 0.03 | 0.02 | 0.02 | 0.02 | 0.01 | 0.19 | 0.28 |
| $\%T_1 > 90\%$ | MSE | 0.08 | -0.02 | 0.02 | 0.00 | 0.04 | 0.00 | 0.01 | -0.01 | -0.01 | -0.01 | -0.02 | -0.15 |
| | MAE | 0.24 | 0.21 | 0.22 | 0.09 | 0.07 | 0.03 | 0.03 | 0.02 | 0.02 | 0.01 | 0.21 | 0.24 |
| $\%T_1 < 90\%$ | MSE | 0.30 | 0.11 | 0.20 | 0.05 | 0.16 | 0.06 | 0.06 | 0.03 | 0.01 | 0.01 | 0.11 | -0.15 |
| | MAE | 0.33 | 0.17 | 0.20 | 0.17 | 0.16 | 0.06 | 0.06 | 0.04 | 0.03 | 0.03 | 0.17 | 0.16 |

# S5 Basis set extrapolation with 6-31+G(d)

Below we list the CC3/6-31+G(d), CCSDT/6-31+G(d), and CCSDTQ/6-31+G(d) data for the states for which CCSDT/*aug*-cc-pVTZ, and CCSDTQ/*aug*-cc-pVTZ results were obtained.

Table S8: Additional CC results obtained with the compact 6-31+G(d) atomic basis set. All values are in eV.

| | | CC3 | CCSDT | CCSDTQ |
|---|---|---|---|---|
| Acetaldehyde | $^1A''(\mathrm{V}; n \to \pi^\star)$ | 4.39 | 4.37 | |
| | $^3A''(\mathrm{V}; n \to \pi^\star)$ | 4.04 | 4.02 | |
| Acetylene | $^1\Sigma_u^-(\mathrm{V}; \pi \to \pi^\star)$ | 7.40 | 7.40 | 7.40 |
| | $^1\Delta_u(\mathrm{V}; \pi \to \pi^\star)$ | 7.72 | 7.73 | 7.73 |
| | $^3\Sigma_u^+(\mathrm{V}; \pi \to \pi^\star)$ | 5.49 | 5.51 | |
| | $^3\Delta_u(\mathrm{V}; \pi \to \pi^\star)$ | 6.57 | 6.57 | 6.57 |
| | $^3\Sigma_u^-(\mathrm{V}; \pi \to \pi^\star)$ | 7.28 | 7.28 | 7.28 |
| | $^1A_u[\mathrm{F}](\mathrm{V}; \pi \to \pi^\star)$ | 3.83 | 3.85 | 3.84 |
| | $^1A_2[\mathrm{F}](\mathrm{V}; \pi \to \pi^\star)$ | 4.05 | 4.07 | 4.06 |
| Ammonia | $^1A_2(\mathrm{R}; n \to 3s)$ | 6.96 | 6.95 | 6.96 |
| | $^1E(\mathrm{R}; n \to 3p)$ | 8.95 | 8.95 | 8.96 |
| | $^1A_1(\mathrm{R}; n \to 3p)$ | 10.19 | 10.19 | 10.20 |
| | $^1A_2(\mathrm{R}; n \to 4s)$ | 11.65 | 11.64 | 11.64 |
| | $^3A_2(\mathrm{R}; n \to 3s)$ | 6.49 | 6.49 | 6.50 |
| Carbon monoxyde | $^1\Pi(\mathrm{V}; n \to \pi^\star)$ | 8.66 | 8.67 | 8.66 |
| | $^1\Sigma^-(\mathrm{V}; \pi \to \pi^\star)$ | 10.19 | 10.13 | 10.12 |
| | $^1\Delta(\mathrm{V}; \pi \to \pi^\star)$ | 10.28 | 10.23 | 10.22 |
| | $^1\Sigma^+(\mathrm{R})$ | 10.89 | 10.92 | 10.90 |
| | $^1\Sigma^+(\mathrm{R})$ | 11.53 | 11.57 | 11.56 |
| | $^1\Pi(\mathrm{R})$ | 11.83 | 11.86 | 11.85 |
| | $^3\Pi(\mathrm{V}; n \to \pi^\star)$ | 6.35 | 6.34 | 6.32 |
| | $^3\Sigma^+(\mathrm{V}; \pi \to \pi^\star)$ | 8.49 | 8.47 | 8.48 |
| | $^3\Delta(\mathrm{V}; \pi \to \pi^\star)$ | 9.44 | 9.39 | 9.40 |
| | $^3\Sigma^-(\mathrm{V}; \pi \to \pi^\star)$ | 9.94 | | |
| | $^3\Sigma^+(\mathrm{R})$ | 10.33 | 10.36 | 10.35 |
| Cyclopropene | $^1B_1(\mathrm{V}; \sigma \to \pi^\star)$ | 6.86 | 6.85 | |
| | $^1B_2(\mathrm{V}; \pi \to \pi^\star)$ | 6.98 | 6.99 | |
| | $^3B_2(\mathrm{V}; \pi \to \pi^\star)$ | 4.37 | 4.38 | |
| | $^3B_1(\mathrm{V}; \sigma \to \pi^\star)$ | 6.61 | 6.60 | |
| Diazomethane | $^1A_2(\mathrm{V}; \pi \to \pi^\star)$ | 3.05 | 3.05 | |
| | $^1B_1(\mathrm{R}; \pi \to 3s)$ | 5.37 | 5.40 | |
| | $^1A_1(\mathrm{V}; \pi \to \pi^\star)$ | 5.83 | 5.86 | |
| | $^3A_2(\mathrm{V}; \pi \to \pi^\star)$ | 2.80 | 2.80 | |
| | $^3A_1(\mathrm{V}; \pi \to \pi^\star)$ | 4.02 | 4.01 | |
| | $^3B_1(\mathrm{R}; \pi \to 3s)$ | 5.20 | 5.23 | |
| | $^3A_1(\mathrm{R}; \pi \to 3p)$ | 6.86 | 6.86 | |

Continued on next page

| | | CC3 | CCSDT | CCSDTQ |
|---|---|---|---|---|
| | $^1A''$[F](V; $\pi \rightarrow \pi^\star$) | 0.62 | 0.60 | |
| Dinitrogen | $^1\Pi_g$(V; $n \rightarrow \pi^\star$) | 9.46 | 9.44 | 9.43 |
| | $^1\Sigma_u^-$(V; $\pi \rightarrow \pi^\star$) | 10.10 | 10.10 | 10.10 |
| | $^1\Delta_u$(V; $\pi \rightarrow \pi^\star$) | 10.47 | 10.48 | 10.47 |
| | $^1\Sigma_g^+$(R) | 13.29 | 13.26 | 13.23 |
| | $^1\Pi_u$(R) | 13.44 | 13.32 | 13.28 |
| | $^1\Sigma_u^+$(R) | 13.51 | 13.51 | 13.48 |
| | $^1\Pi_u$(R) | 13.85 | 13.82 | 13.79 |
| | $^3\Sigma_u^+$(V; $\pi \rightarrow \pi^\star$) | 7.68 | 7.68 | 7.70 |
| | $^3\Pi_g$(V; $n \rightarrow \pi^\star$) | 8.10 | 8.09 | 8.08 |
| | $^3\Delta_u$(V; $\pi \rightarrow \pi^\star$) | 8.99 | 8.99 | 8.99 |
| | $^3\Sigma_u^-$(V; $\pi \rightarrow \pi^\star$) | 9.80 | 9.78 | 9.77 |
| Ethylene | $^1B_{3u}$(R; $\pi \rightarrow 3s$) | 7.72 | 7.73 | 7.72 |
| | $^1B_{1u}$(V; $\pi \rightarrow \pi^\star$) | 8.14 | 8.15 | 8.14 |
| | $^1B_{1g}$(R; $\pi \rightarrow 3p$) | 8.29 | 8.30 | 8.29 |
| | $^3B_{1u}$(V; $\pi \rightarrow \pi^\star$) | 4.52 | 4.53 | 4.53 |
| | $^3B_{3u}$(R; $\pi \rightarrow 3s$) | 7.49 | 7.51 | 7.51 |
| | $^3B_{1g}$(R; $\pi \rightarrow 3p$) | 8.20 | 8.22 | 8.22 |
| Formaldehyde | $^1A_2$(V; $n \rightarrow \pi^\star$) | 4.03 | 4.01 | 4.02 |
| | $^1B_2$(R; $n \rightarrow 3s$) | 7.24 | 7.23 | 7.28 |
| | $^1B_2$(R; $n \rightarrow 3p$) | 8.02 | 8.01 | 8.04 |
| | $^1A_1$(R; $n \rightarrow 3p$) | 8.30 | 8.29 | 8.34 |
| | $^1A_2$(R; $n \rightarrow 3p$) | 8.70 | 8.68 | 8.72 |
| | $^1B_1$(V; $\sigma \rightarrow \pi^\star$) | 9.37 | 9.34 | 9.35 |
| | $^1A_1$(V; $\pi \rightarrow \pi^\star$) | 9.83 | 9.83 | 9.78 |
| | $^3A_2$(V; $n \rightarrow \pi^\star$) | 3.66 | 3.65 | 3.66 |
| | $^3A_1$(V; $\pi \rightarrow \pi^\star$) | 6.09 | 6.09 | 6.10 |
| | $^3B_2$(R; $n \rightarrow 3s$) | 7.07 | 7.06 | 7.11 |
| | $^3B_2$(R; $n \rightarrow 3p$) | 7.84 | 7.82 | 7.86 |
| | $^3A_1$(R; $n \rightarrow 3p$) | 8.17 | 8.15 | 8.20 |
| | $^3B_1$(R; $n \rightarrow 3d$) | 8.54 | 8.52 | 8.53 |
| | $^1A$"[F](V; $n \rightarrow \pi^\star$) | 2.88 | 2.85 | 2.86 |
| Formamide | $^1A''$V; ($n \rightarrow \pi^\star$) | 5.83 | 5.79 | |
| | $^3A''$(V; $n \rightarrow \pi^\star$) | 5.55 | 5.52 | |
| | $^3A'$(V; $\pi \rightarrow \pi^\star$) | 5.92 | 5.90 | |
| Hydrogen chloride | $^1\Pi$(CT) | 7.84 | 7.84 | 7.84 |
| Hydrogen sulfide | $^1A_2$(R; $n \rightarrow 4p$) | 6.47 | 6.46 | 6.46 |
| | $^1B_1$(R; $n \rightarrow 4s$) | 6.05 | 6.05 | 6.05 |
| | $^3A_2$(R; $n \rightarrow 4p$) | 6.01 | 6.00 | 6.00 |
| | $^3B_1$(R; $n \rightarrow 4s$) | 5.66 | 5.66 | 5.66 |
| Ketene | $^1A_2$(V; $\pi \rightarrow \pi^\star$) | 3.86 | 3.85 | |
| | $^1B_1$(R; $n \rightarrow 3s$) | 5.91 | 5.94 | |
| | $^1A_2$(R; $\pi \rightarrow 3p$) | 7.34 | 7.38 | |
| | $^3A_2$(V; $n \rightarrow \pi^\star$) | 3.78 | 3.78 | |
| | $^3A_1$(V; $\pi \rightarrow \pi^\star$) | 5.63 | 5.62 | |
| | $^3B_1$(R; $n \rightarrow 3s$) | 5.68 | 5.70 | |

Continued on next page

| | | CC3 | CCSDT | CCSDTQ |
|---|---|---|---|---|
| | $^3A_2(\mathrm{R}; \pi \to 3p)$ | 7.27 | 7.31 | |
| | $^1A$"[F]$(\mathrm{V}; \pi \to \pi^\star)$ | 0.90 | 0.90 | |
| Methanimine | $^1A$"$(\mathrm{V}; n \to \pi^\star)$ | 5.34 | 5.32 | 5.33 |
| | $^3A$"$(\mathrm{V}; n \to \pi^\star)$ | 4.72 | 4.71 | 4.72 |
| Nitrosomethane | $^1A''(\mathrm{V}; n \to \pi^\star)$ | 2.02 | 2.00 | |
| | $^1A'(\mathrm{R}; n \to 3s/3p)$ | 6.49 | 6.48 | |
| | $^3A''(\mathrm{V}; n \to \pi^\star)$ | 1.14 | 1.13 | |
| | $^3A'(\mathrm{V}; \pi \to \pi^\star)$ | 5.55 | 5.55 | |
| | $^1A''$[F]$(\mathrm{V}; n \to \pi^\star)$ | 1.72 | 1.70 | |
| Streptocyanine | $^1B_2(\mathrm{V}; \pi \to \pi^\star)$ | 7.28 | 7.25 | |
| | $^3B_2(\mathrm{V}; \pi \to \pi^\star)$ | 5.53 | 5.52 | |
| Thioformaldehyde | $^1A_2(\mathrm{V}; n \to \pi^\star)$ | 2.26 | 2.24 | 2.25 |
| | $^1B_2(\mathrm{R}; n \to 4s)$ | 5.88 | 5.88 | 5.89 |
| | $^1A_1(\mathrm{V}; \pi \to \pi^\star)$ | 6.82 | 6.79 | 6.71 |
| | $^3A_2(\mathrm{V}; n \to \pi^\star)$ | 1.98 | 1.97 | 1.97 |
| | $^3A_1(\mathrm{V}; \pi \to \pi^\star)$ | 3.38 | 3.39 | 3.39 |
| | $^3B_2(\mathrm{R}; n \to 4s)$ | 5.67 | 5.67 | 5.69 |
| | $^1A_2$[F]$(\mathrm{V}; n \to \pi^\star)$ | 1.99 | 1.96 | 1.96 |
| Water | $^1B_1(\mathrm{R}; n \to 3s)$ | 8.32 | 8.32 | 8.33 |
| | $^1A_2(\mathrm{R}; n \to 3p)$ | 10.74 | 10.73 | 10.74 |
| | $^1A_1(\mathrm{R}; n \to 3s)$ | 10.84 | 10.83 | 10.84 |
| | $^3B_1(\mathrm{R}; n \to 3s)$ | 7.71 | 7.70 | 7.71 |
| | $^3A_2(\mathrm{R}; n \to 3p)$ | 10.34 | 10.33 | 10.34 |
| | $^3A_1(\mathrm{R}; n \to 3s)$ | 10.16 | 10.15 | 10.17 |

# S6 sCI and exFCI results

Table S9: Vertical excitations (in eV) for various states of the studied molecules computed with a extrapolated sCI method (exFCI). The number of determinants $N_{\text{det}}$ of the largest sCI wave functions and their corresponding excitation energies are also reported.

| Molecule | Transition | AVDZ | | | AVTZ | | | AVQZ | | |
|---|---|---|---|---|---|---|---|---|---|---|
| | | $N_{\text{det}}$ | sCI | exFCI | $N_{\text{det}}$ | sCI | exFCI | $N_{\text{det}}$ | sCI | exFCI |
| Acetaldehyde | $^1A''(n \to \pi^\star)$ | 5 803 234 | 4.37 | 4.34 | 1 357 186 | 4.29 | 4.31 | | | |
| | $^3A''(n \to \pi^\star)$ | 4 151 858 | 4.07 | 3.98 | 1 722 025 | 3.51 | 4.01 | | | |
| Acetylene | $^1\Sigma_u^-(\pi \to \pi^\star)$ | 4 162 848 | 7.21 | 7.20 | 3 113 480 | 7.09 | 7.10 | | | |
| | $^1\Delta_u(\pi \to \pi^\star)$ | | 7.52 | 7.51 | | 7.43 | 7.44 | | | |
| | $^3\Sigma_u^+(\pi \to \pi^\star)$ | 8 494 075 | 5.50 | 5.50 | 3 282 690 | 5.52 | 5.53 | | | |
| | $^3\Delta_u(\pi \to \pi^\star)$ | 4 403 434 | 6.46 | 6.46 | 2 190 673 | 6.40 | 6.40 | | | |
| | $^3\Sigma_u^-(\pi \to \pi^\star)$ | | 7.14 | 7.14 | | 7.08 | 7.08 | | | |
| | $^1A_u(\pi \to \pi^\star)$ [F] | 5 943 690 | 3.71 | 3.71 | 3 982 131 | 3.64 | 3.64 | | | |
| | $^1A_2(\pi \to \pi^\star)$ [F] | 5 788 835 | 3.93 | 3.93 | 3 967 196 | 3.85 | 3.85 | | | |
| Ammonia | $^1A_2(n \to 3s)$ | 2 063 356 | 6.48 | 6.48 | 6 450 032 | 6.59 | 6.59 | 3 608 385 | 6.64 | 6.64 |
| | $^1E(n \to 3p)$ | | 8.08 | 8.08 | | 8.17 | 8.16 | | 8.21 | 8.22 |
| | $^1A_1(n \to 3p)$ | | 9.68 | 9.68 | | 9.34 | 9.33 | | 9.14 | 9.14 |
| | $^1A_2(n \to 4s)$ | | 10.41 | 10.41 | | 9.96 | 9.96 | | | |
| | $^3A_1(n \to 3s)$ | 2 389 435 | 6.19 | 6.19 | 6 171 274 | 6.31 | 6.31 | 2 698 282 | 6.34 | 6.35 |
| Carbon monoxide | $^1\Pi(n \to \pi^\star)$ | 375 543 | 8.56 | 8.57 | 6 832 118 | 8.46 | 8.49 | 5 809 330 | 8.41 | 8.50 |
| | $^1\Sigma(\pi \to \pi^\star)$ | | 10.07 | 10.05 | | 9.93 | 9.92 | | 9.92 | 9.99 |
| | $^1\Delta(\pi \to \pi^\star)$ | | 10.18 | 10.16 | | 10.06 | 10.06 | | 10.04 | 10.11 |
| | $^1\Sigma^+$(R) | | 10.93 | 10.94 | | 10.95 | 10.95 | | 10.89 | 10.96 |
| | $^1\Sigma^+$(R) | | 11.52 | 11.52 | | 11.51 | 11.52 | | 11.46 | 11.53 |
| | $^1\Pi$(R) | | 11.76 | 11.76 | | 11.70 | 11.72 | | 11.64 | 11.70 |
| | $^3\Pi(n \to \pi^\star)$ | 1 238 764 | 6.28 | 6.29 | 2 221 825 | 6.28 | 6.28 | 4 054 250 | 6.28 | 6.29 |
| | $^3\Sigma^+(\pi \to \pi^\star)$ | 2 117 552 | 8.46 | 8.46 | 7 820 835 | 8.46 | 8.45 | 2 302 698 | 8.49 | 8.49 |
| | $^3\Delta(\pi \to \pi^\star)$ | | 9.34 | 9.33 | | 9.28 | 9.27 | | 9.29 | 9.29 |
| | $^3\Sigma^-(\pi \to \pi^\star)$ | | 9.84 | 9.83 | | 9.78 | 9.80 | | 9.77 | 9.78 |
| | $^3\Sigma^+$(R) | | 10.42 | 10.41 | | 10.49 | 10.47 | | | |
| Cyclopropene | $^1B_1(\sigma \to \pi^\star)$ | 5 496 693 | 6.75 | 6.7[a] | 4 594 382 | 6.61 | 6.6[a] | | | |
| | $^1B_2(\pi \to \pi^\star)$ | | 6.82 | 6.82 | | 6.69 | 6.7[a] | | | |
| | $^3B_2(\pi \to \pi^\star)$ | 5 484 297 | 4.39 | 4.35 | 1 762 752 | 4.38 | 4.38 | | | |
| | $^3B_1(\sigma \to \pi^\star)$ | 4 457 619 | 6.44 | 6.43 | 2 705 402 | 6.44 | 6.45 | | | |
| Diazomethane | $^1A_2(\pi \to \pi^\star)$ | 8 373 270 | 3.08 | 3.09 | 4 366 276 | 2.99 | 3.14 | | | |
| | $^1B_1(\pi \to 3s)$ | | 5.38 | 5.35 | | 5.51 | 5.54 | | | |
| | $^1A_1(\pi \to \pi^\star)$ | | 5.82 | 5.79 | | 5.83 | 5.90 | | | |
| | $^3A_2(\pi \to \pi^\star)$ | 3 407 311 | 2.81 | 2.81 | 1 887 903 | 2.58 | 2.8[a] | | | |
| | $^3A_1(\pi \to \pi^\star)$ | | 4.05 | 4.03 | | 3.81 | 4.05 | | | |
| | $^3B_1(\pi \to 3s)$ | | 5.24 | 5.18 | | 5.22 | 5.35 | | | |
| | $^3A_1(\pi \to 3p)$ | | 6.85 | 6.81 | | 6.65 | 6.82 | | | |
| | $^1A''(\pi \to \pi^\star)$ [F] | 10 654 552 | 0.65 | 0.65 | 2 325 176 | 0.60 | 0.71 | | | |
| Dinitrogen | $^1\Pi_g(n \to 3s)$ | 2 775 773 | 9.41 | 9.41 | 2 545 210 | 9.32 | 9.34 | 1 728 899 | 9.28 | 9.34 |
| | $^1\Sigma_u^-(\pi \to \pi^\star)$ | | 10.05 | 10.05 | | 9.89 | 9.88 | | 9.82 | 9.92 |
| | $^1\Delta_u^-(\pi \to \pi^\star)$ | | 10.43 | 10.43 | | 10.29 | 10.29 | | 10.24 | 10.31 |
| | $^1\Sigma_g^+$(R) | | 13.19 | 13.18 | | 12.98 | 12.98 | | 12.85 | 12.89 |
| | $^1\Pi_u$(R) | | 13.12 | 13.12 | | 13.12 | 13.03 | | 13.12 | 13.1[a] |
| | $^1\Sigma_u^+$(R) | | 13.11 | 13.11 | | 13.10 | 13.09 | | 13.20 | 13.2[a] |
| | $^1\Pi_u$(R) | | 13.56 | 13.56 | | 13.39 | 13.46 | | 13.23 | 13.7[a] |
| | $^3\Sigma_u^+(\pi \to \pi^\star)$ | 8 139 401 | 7.70 | 7.70 | 3 302 015 | 7.70 | 7.70 | 4 881 350 | 7.73 | 7.74 |
| | $^3\Pi_g(n \to \pi^\star)$ | 2 705 349 | 8.05 | 8.05 | 6 298 290 | 8.01 | 8.01 | 2 530 197 | 8.04 | 8.03 |

Continued on next page

| Molecule | Transition | AVDZ | | | AVTZ | | | AVQZ | | |
|---|---|---|---|---|---|---|---|---|---|---|
| | | $N_{\text{det}}$ | sCI | exFCI | $N_{\text{det}}$ | sCI | exFCI | $N_{\text{det}}$ | sCI | exFCI |
| | $^3\Delta_u(\pi \to \pi^\star)$ | | 8.96 | 8.96 | | 8.87 | 8.87 | | 8.88 | 8.88 |
| | $^3\Sigma_u^-(\pi \to \pi^\star)$ | | 9.75 | 9.75 | | 9.66 | 9.66 | | 9.67 | 9.66 |
| Ethylene | $^1B_{3u}(\pi \to 3s)$ | 4 158 361 | 7.32 | 7.31 | 11 069 830 | 7.38 | 7.39 | | | |
| | $^1B_{1u}(\pi \to \pi^\star)$ | | 7.94 | 7.93 | | 7.90 | 7.93 | | | |
| | $^1B_{1g}(\pi \to 3p)$ | | 8.01 | 8.00 | | 8.06 | 8.08 | | | |
| | $^3B_{1u}(\pi \to \pi^\star)$ | 3 767 429 | 4.55 | 4.55 | 1 709 107 | 4.55 | 4.54 | | | |
| | $^3B_{3u}(\pi \to 3s)$ | 8 479 296 | 7.23 | 7.16 | 4 055 685 | 7.55 | [a] | | | |
| | $^3B_{1g}(\pi \to 3p)$ | | 8.00 | 7.93 | | 8.32 | [a] | | | |
| Formaldehyde | $^1A_2(n \to \pi^\star)$ | 2 043 030 | 4.00 | 3.99 | 6 773 751 | 3.97 | 3.98 | | | |
| | $^1B_2(n \to 3s)$ | | 7.15 | 7.11 | | 7.24 | 7.23 | | | |
| | $^1B_2(n \to 3p)$ | | 8.09 | 8.04 | | 8.14 | 8.13 | | | |
| | $^1A_1(n \to 3p)$ | | 8.15 | 8.12 | | 8.24 | 8.23 | | | |
| | $^1A_2(n \to 3p)$ | | 8.74 | 8.65 | | 8.68 | 8.67 | | | |
| | $^1B_1(\sigma \to \pi^\star)$ | | 9.32 | 9.29 | | 9.20 | 9.22 | | | |
| | $^1A_1(\pi \to \pi^\star)$ | | 9.60 | 9.53 | | 9.47 | 9.43 | | | |
| | $^3A_2(n \to \pi^\star)$ | 10 774 489 | 3.58 | 3.58 | 5 289 475 | 3.58 | 3.58 | | | |
| | $^3A_1(\pi \to \pi^\star)$ | 4 192 682 | 6.10 | 6.10 | 6 637 572 | 6.06 | 6.06 | | | |
| | $^3B_2(n \to 3s)$ | | 6.96 | 6.95 | | 7.09 | 7.06 | | | |
| | $^3B_2(n \to 3p)$ | | 7.88 | 7.87 | | 7.98 | 7.94 | | | |
| | $^3A_1(n \to 3p)$ | | 8.02 | 8.01 | | 8.13 | 8.10 | | | |
| | $^3B_1(n \to 3d)$ | | 8.48 | 8.48 | | 8.43 | 8.42 | | | |
| | $^1A''(n \to \pi^\star)$ [F] | 6 989 511 | 2.86 | 2.86 | 5 289 475 | 2.83 | 2.80 | | | |
| Formamide | $^1A''(n \to \pi^\star)$ | 6 392 357 | 5.74 | 5.70 | 5 249 511 | 5.65 | 5.7[a] | | | |
| | $^1A'(n \to 3s)$ | | 6.76 | 6.67 | | | | | | |
| | $^1A'(n \to \pi^\star)$ | | 7.73 | 7.64 | | 7.64 | 7.63 | | | |
| | $^3A''(n \to \pi^\star)$ | 3 958 975 | 5.44 | 5.42 | 1 791 542 | 5.37 | 5.4[a] | | | |
| | $^3A'(\pi \to \pi^\star)$ | 3 452 920 | 5.90 | 5.82 | 1 791 542 | 5.65 | 5.7[a] | | | |
| Hydrogen chloride | $^1\Pi(\text{CT})$ | 1 049 127 | 7.82 | 7.82 | 3 546 637 | 7.84 | 7.84 | 6 944 492 | 7.88 | 7.88 |
| Hydrogen sulfide | $^1A_2(n \to 4p)$ | 2 005 501 | 6.29 | 6.29 | 5 354 721 | 6.18 | 6.18 | | | |
| | $^1B_1(n \to 4s)$ | | 6.10 | 6.10 | | 6.24 | 6.24 | | | |
| | $^3A_2(n \to 4p)$ | 4 293 448 | 5.90 | 5.90 | 5 696 382 | 5.81 | 5.81 | | | |
| | $^3B_1(n \to 4s)$ | 2 401 216 | 5.75 | 5.75 | 3 647 563 | 5.89 | 5.89 | | | |
| Ketene | $^1A_2(\pi \to \pi^\star)$ | 6 698 206 | 3.87 | 3.84 | 4 648 503 | 3.83 | 3.86 | | | |
| | $^1B_1(n \to 3s)$ | | 5.96 | 5.88 | | 6.04 | 6.01 | | | |
| | $^1A_2(\pi \to 3p)$ | | 7.12 | 7.08 | | 7.22 | 7.18 | | | |
| | $^3A_2(n \to \pi^\star)$ | 3 293 583 | 3.81 | 3.79 | 1 850 086 | 3.59 | 3.77 | | | |
| | $^3A_1(\pi \to \pi^\star)$ | | 5.67 | 5.64 | | 5.44 | 5.61 | | | |
| | $^3B_1(n \to 3s)$ | | 5.75 | 5.68 | | 5.70 | 5.79 | | | |
| | $^3A_2(\pi \to 3p)$ | | 7.11 | 7.07 | | 7.02 | 7.12 | | | |
| | $^1A''(\pi \to \pi^\star)$ [F] | 4 289 184 | 0.96 | 0.96 | 2 798 757 | 0.94 | 1.00 | | | |
| Methanimine | $^1A''(n \to \pi^\star)$ | 2 526 499 | 5.25 | 5.25 | 5 096 976 | 5.20 | 5.23 | | | |
| | $^3A''(n \to \pi^\star)$ | 1 861 136 | 4.63 | 4.63 | 3 954 983 | 4.56 | 4.65 | | | |
| Nitrosomethane | $^1A''(n \to \pi^\star)$ | 3 446 151 | 2.00 | 1.99 | 4 270 321 | 1.89 | 2.0[a] | | | |
| | $^1A'(n, n \to \pi^\star, \pi^\star)$ | | 4.82 | 4.81 | 5 285 063 | 4.72 | 4.72 | | | |
| | $^1A'(n \to 3s/3p)$ | | 6.34 | 6.29 | | 6.34 | 6.4[a] | | | |
| | $^3A''(n \to \pi^\star)$ | 4 079 674 | 1.14 | 1.15 | 1 607 335 | 1.09 | 1.16 | | | |
| | $^3A'(\pi \to \pi^\star)$ | 3 225 628 | 5.61 | 5.56 | 1 792 165 | 5.60 | 5.60 | | | |
| | $^1A''(n \to \pi^\star)$ [F] | 4 509 295 | 1.70 | 1.70 | 2 718 837 | 1.62 | 1.7[a] | | | |
| Streptocyanine-C1 | $^1B_2(\pi \to \pi^\star)$ | 8 620 009 | 7.17 | 7.14 | 5 468 384 | 7.07 | 7.1[a] | | | |
| | $^3B_2(\pi \to \pi^\star)$ | 6 970 063 | 5.52 | 5.47 | 2 436 373 | 5.51 | 5.52 | | | |
| Thioformaldehyde | $^1A_2(n \to \pi^\star)$ | 2 672 140 | 2.26 | 2.26 | 6 036 063 | 2.21 | 2.22 | | | |
| | $^1B_2(n \to 4s)$ | | 5.85 | 5.83 | | 5.97 | 5.96 | | | |

Continued on next page

| Molecule | Transition | AVDZ | | | AVTZ | | | AVQZ | | |
|---|---|---|---|---|---|---|---|---|---|---|
| | | $N_{\text{det}}$ | sCI | exFCI | $N_{\text{det}}$ | sCI | exFCI | $N_{\text{det}}$ | sCI | exFCI |
| | $^1A_1(\pi \rightarrow \pi^\star)$ | | 6.54 | 6.5[a] | | 6.40 | 6.4[a] | | | |
| | $^3A_2(n \rightarrow \pi^\star)$ | 1 841 330 | 1.96 | 1.97 | 4 611 888 | 1.93 | 1.94 | | | |
| | $^3A_1(\pi \rightarrow \pi^\star)$ | 8 450 984 | 3.43 | 3.45 | 4 169 151 | 3.40 | 3.43 | | | |
| | $^3B_2(n \rightarrow 4s)$ | | 5.68 | 5.66 | | 5.66 | 5.6[a] | | | |
| | $^1A_2(n \rightarrow \pi^\star)$ [F] | 245 005 | 1.98 | 1.98 | 6 108 383 | 1.94 | 1.95 | | | |
| Water | $^1B_1(n \rightarrow 3s)$ | 5 869 449 | 7.53 | 7.53 | 5 589 200 | 7.63 | 7.62 | 1 139 302 | 7.69 | 7.68 |
| | $^1A_2(n \rightarrow 3p)$ | | 9.32 | 9.32 | | 9.41 | 9.41 | | 9.46 | 9.46 |
| | $^1A_1(n \rightarrow 3s)$ | | 9.94 | 9.94 | | 9.99 | 9.99 | | 10.04 | 10.02 |
| | $^3B_1(n \rightarrow 3s)$ | 1 985 139 | 7.14 | 7.14 | 5 950 423 | 7.25 | 7.25 | 2 342 816 | 7.30 | 7.30 |
| | $^3A_2(n \rightarrow 3p)$ | 4 566 873 | 9.14 | 9.14 | 3 760 373 | 9.24 | 9.24 | 525 499 | 9.28 | 9.28 |
| | $^3A_1(n \rightarrow 3s)$ | | 9.49 | 9.49 | | 9.54 | 9.54 | | 9.58 | 9.58 |

[a] CI convergence too slow to provide reliable estimate.

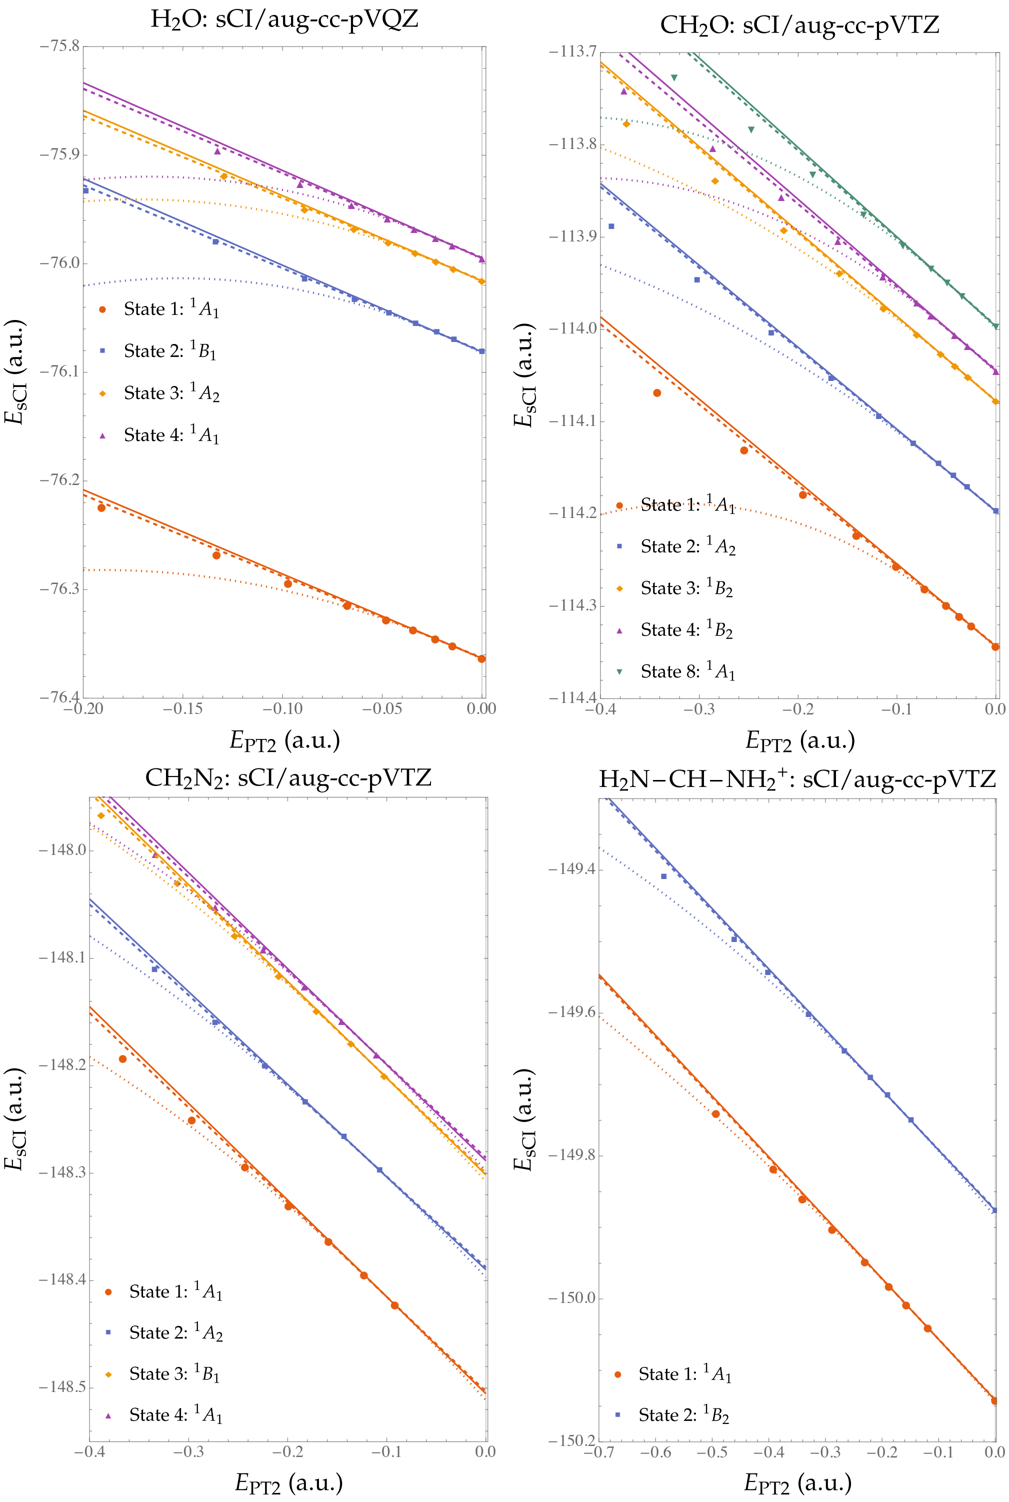


Figure S1: sCI energy $E_{\text{sCI}}$ (in a.u.) as a function of the second-order perturbative correction $E_{\text{PT2}}$ (in a.u.) for various singlet states of water ($H_2O$), formaldehyde ($CH_2O$), diazomethane ($CH_2N_2$) and streptocyanine-C1 ($H_2N{-}CH{-}NH_2{}^+$). The extrapolation to the FCI limit corresponds to $E_{\text{PT2}} = 0$. Several extrapolations are reported: i) two-point linear fit (solid slides), ii) three-point linear fit (dashed lines), and iii) three-point quadratic fit (dotted lines). The raw data are reported in Table S10.

Table S10: Total energies (in a.u.) and excitation energies (in eV) of several singlet states of water, formaldehyde, diazomethane and streptocyanine-C1 for various extrapolations: i) two-point linear fit, ii) three-point linear fit, and iii) three-point quadratic fit.

| Molecule | Basis | State | Total energies (a.u.) | | | Excitation energies (eV) | | |
|---|---|---|---|---|---|---|---|---|
| | | | 2-point linear | 3-point linear | 3-point quadratic | 2-point linear | 3-point linear | 3-point quadratic |
| Water | aug-cc-pVQZ | $^1A_1$ | −76.363 312 | −76.362 851 | −76.364088 | — | — | — |
| | | $^1B_1$ | −76.081 152 | −76.080 586 | −76.082105 | 7.68 | 7.68 | 7.67 |
| | | $^1A_2$ | −76.015 753 | −76.015 753 | −76.016592 | 9.46 | 9.46 | 9.46 |
| | | $^1A_1$ | −75.994 943 | −75.994 943 | −75.995900 | 10.02 | 10.01 | 10.02 |
| Formaldehyde | aug-cc-pVTZ | $^1A_1$ | −114.343 322 | −114.342 705 | −114.342924 | — | — | — |
| | | $^1A_2$ | −114.196 920 | −114.196 578 | −114.197313 | 3.98 | 3.98 | 3.96 |
| | | $^1B_2$ | −114.077 546 | −114.077 213 | −114.078352 | 7.23 | 7.22 | 7.20 |
| | | $^1B_2$ | −114.044 721 | −114.043 658 | −114.034962 | 8.13 | 8.14 | 8.38 |
| | | $^1A_1$ | −114.041 033 | −114.039 965 | −114.044155 | 8.23 | 8.24 | 8.13 |
| | | $^1A_2$ | −114.024 737 | −114.024 398 | −114.025248 | 8.67 | 8.66 | 8.64 |
| | | $^1B_1$ | −114.004 606 | −114.004 206 | −114.004960 | 9.22 | 9.21 | 9.20 |
| | | $^1A_1$ | −113.996 698 | −113.995 874 | −113.998357 | 9.43 | 9.44 | 9.38 |
| Diazomethane | aug-cc-pVTZ | $^1A_1$ | −148.505 218 | −148.503 165 | −148.511381 | — | — | — |
| | | $^1A_2$ | −148.389 825 | −148.387 654 | −148.396857 | 3.14 | 3.14 | 3.12 |
| | | $^1B_1$ | −148.301 533 | −148.299 769 | −148.307723 | 5.54 | 5.53 | 5.54 |
| | | $^1A_1$ | −148.288 384 | −148.285 649 | −148.297847 | 5.90 | 5.92 | 5.81 |
| Strepto-cyanine-C1 | aug-cc-pVTZ | $^1A_1$ | −150.141 796 | −150.141 081 | −150.145 289 | — | — | — |
| | | $^1B_2$ | −149.876 489 | −149.875 113 | −149.884 967 | 7.22 | 7.24 | 7.08 |
